# Supplementary material for: Identification of Gaussian Process State Space Models
Source: arXiv:1705.10888 source file (2017-11-07)
Supplement: Supplementary file 1 [file tikz_samples_ep-14-all.tex]

\definecolor{color0}{rgb}{0.12156862745098,0.466666666666667,0.705882352941177}
\definecolor{color1}{rgb}{1,0.498039215686275,0.0549019607843137}

\begin{groupplot}[group style={group size=1 by 3}]
\nextgroupplot[
xshift=-8,
title={14 episodes},
title style={font=\large},
xmin=-1.45, xmax=30.45,
ymin=2.7, ymax=6.7,
width=\figurewidth,
height=\figureheight,
xtick={},
xticklabels={},
yticklabels={},
tick align=outside,
tick pos=left,
x grid style={white!69.019607843137251!black},
y grid style={white!69.019607843137251!black}
]
\addplot [semithick, color0, opacity=0.3]
table {%
0 3.40958979204541
1 3.50167738560338
2 3.46529177834903
3 3.17787007728519
4 2.96321605330536
5 3.25713313015265
6 4.02396255002326
7 4.71678585673224
8 5.02128474732438
9 5.10964208769495
10 5.18783930452376
11 5.07931112500971
12 4.63434035448156
13 4.26531348004429
14 3.64034226099943
15 3.15325890209546
16 2.48823453461459
17 2.01620910123989
18 2.15800268261965
19 2.56798940848056
20 2.94205950842422
21 3.1773958046763
22 3.45997202785605
23 3.39455919879405
24 3.3109822116968
25 2.91119484821375
26 2.44161033553841
27 1.92131263264334
28 1.38746441779804
29 0.75519039884928
};
\addplot [semithick, color0, opacity=0.3]
table {%
0 3.42699982278861
1 3.57593501289551
2 3.54534445536686
3 3.16367232221292
4 2.89351097212513
5 3.22218827523777
6 3.77073000432696
7 4.19101251472082
8 4.83605807107464
9 5.07627474763137
10 5.38041354711774
11 5.70704345516276
12 5.56890809893928
13 5.23652033163488
14 4.82532051004374
15 4.30221247932572
16 3.73612093299553
17 3.17291588113259
18 2.7751145676743
19 2.39383450738712
20 2.04066982978872
21 2.05616701364223
22 2.24607249272239
23 2.59993370777652
24 2.89567842867222
25 3.13308556715328
26 3.18435125092283
27 2.98279560978564
28 2.7226253621437
29 2.50549064296298
};
\addplot [semithick, color0, opacity=0.3]
table {%
0 3.5687793361235
1 3.64864890144533
2 3.5933144178986
3 3.50631783126456
4 3.3013657346245
5 3.36022913618829
6 3.73008479237651
7 4.2078025262175
8 4.3763448626275
9 4.41568338759936
10 4.31530013183546
11 4.06378541772542
12 3.64266811269897
13 2.93488408642009
14 2.5640596666683
15 2.30803504839574
16 2.07463970749525
17 2.21824033185909
18 2.40603900497724
19 2.64991840812583
20 2.91788603047588
21 3.08886079762311
22 2.95231695772735
23 2.85365665656592
24 2.69799567369068
25 2.55340066617682
26 2.47771400217981
27 2.35030501211684
28 2.17714289447303
29 1.96319759835024
};
\addplot [semithick, color0, opacity=0.3]
table {%
0 3.50917617071343
1 3.62459349701745
2 3.49396195733172
3 3.24063668113275
4 3.03062280404505
5 3.35643676415249
6 3.79378220187777
7 4.34715290371863
8 4.55098428982971
9 4.79778215364053
10 4.88394197786883
11 5.11705167689105
12 4.80260044262643
13 4.40039399738037
14 3.89560085116205
15 3.25011802334636
16 2.63692328489166
17 2.2685214930776
18 2.13343057373282
19 2.2468995387567
20 2.39657794434582
21 2.52704508780836
22 2.62597683642972
23 2.63096126868406
24 2.55799294603502
25 2.39697287668125
26 2.3986920101605
27 2.53716701546458
28 2.51916559554652
29 2.65806924831059
};
\addplot [semithick, color0, opacity=0.3]
table {%
0 3.42957721061187
1 3.62810576110068
2 3.55968106700103
3 3.28028350211976
4 3.08687389624361
5 3.36676063828493
6 3.96470643520351
7 4.65591528259081
8 4.99846550391255
9 5.30379766487492
10 5.40157529643755
11 5.46628451230192
12 5.33315546923832
13 5.16378133734166
14 4.98861257430269
15 4.84269327495638
16 4.56072850362137
17 4.39380200845374
18 4.15652909436142
19 3.86919750811954
20 3.43091537227068
21 2.86869094222625
22 2.4194864777625
23 2.70543330960008
24 3.07318577441776
25 3.27653620149313
26 3.44512794155084
27 3.43301343242384
28 3.19955749072628
29 2.88273362664525
};
\addplot [semithick, color0, opacity=0.3]
table {%
0 3.58271448972532
1 3.60798917542732
2 3.53327194281838
3 3.22550264354267
4 2.93239925116926
5 3.13378987770534
6 3.56026218442165
7 4.01085482849916
8 4.4503807873019
9 4.69027957152752
10 4.95166631659382
11 5.09406065618158
12 5.04044946682854
13 4.82127636248569
14 4.45886796783539
15 4.0002986327193
16 3.61433263260617
17 3.12004475871068
18 2.82427737644011
19 2.81629727830065
20 3.14825632041384
21 3.83175862899455
22 3.99643732888913
23 3.72675738427075
24 3.54434129826608
25 3.33356819409522
26 3.12689446742286
27 2.89450163441023
28 2.583749172733
29 2.29130262076071
};
\addplot [semithick, color0, opacity=0.3]
table {%
0 3.48415351143306
1 3.69972213871165
2 3.60863876418089
3 3.27977813785367
4 3.01928790917842
5 3.23955851527913
6 3.73084252403738
7 4.33828781336935
8 4.77128626926186
9 5.09549283510469
10 5.15793281815051
11 5.13966043308529
12 4.87167117391483
13 4.3480569999695
14 3.70381667178058
15 3.07766671420779
16 2.52045799120353
17 2.65879870516345
18 3.24965094703607
19 3.50899520346757
20 3.72580005897546
21 3.69180057485025
22 3.54799234215003
23 3.443186137911
24 3.02563596850535
25 2.46909977435114
26 2.00560309657981
27 1.75143731878086
28 1.47603284002685
29 1.06218083530241
};
\addplot [semithick, color0, opacity=0.3]
table {%
0 3.43161912746504
1 3.54484184017913
2 3.59141419837195
3 3.36363944965745
4 3.17510763125831
5 3.41696478838067
6 3.87457581291773
7 4.34643643901908
8 4.56820852015325
9 4.56009828529957
10 4.64177392361453
11 4.49484515725723
12 4.32085992532612
13 3.9319482609581
14 3.57007948550353
15 3.13256334463826
16 2.8422667989331
17 2.63788966348012
18 2.77276768827155
19 2.85390266958506
20 2.96744371562682
21 2.96336963929044
22 2.98770548130435
23 3.14725504602689
24 3.21146022586526
25 3.16156047427682
26 3.00467079835681
27 2.98540330491536
28 3.11491803687528
29 3.07835950349473
};
\addplot [semithick, color0, opacity=0.3]
table {%
0 3.33605404983952
1 3.56439158272457
2 3.51708511909016
3 3.27068313491807
4 3.17137612479015
5 3.68281002382575
6 4.06067365583184
7 4.48273406115369
8 4.82036263651631
9 5.30046352927838
10 5.52215848100765
11 5.75901359028889
12 5.59028097901986
13 5.36116049514103
14 4.99096712490994
15 4.74858362995726
16 4.2034230843411
17 3.71952379691762
18 3.17478082829064
19 2.63396781954658
20 2.21992691162308
21 2.12191488803207
22 2.16284916392714
23 2.51070599737012
24 2.97920858690039
25 3.31523809336664
26 3.70491098621841
27 4.05627482797773
28 4.21963114526042
29 4.22066580163399
};
\addplot [semithick, color0, opacity=0.3]
table {%
0 3.46336915001094
1 3.53038469539622
2 3.52998643596527
3 3.23371263929224
4 3.07933815049259
5 3.31888891442268
6 3.65610640818181
7 4.07739885168013
8 4.65275934351464
9 4.94536934880634
10 5.09265397344609
11 5.06960717688256
12 4.99233401632597
13 4.75203411866488
14 4.29119631733133
15 3.81192158284231
16 3.30838290890127
17 2.85336652330844
18 2.47074774235091
19 2.145801813159
20 2.2273660251196
21 2.49072661795598
22 2.66318186803857
23 2.69788449822174
24 2.72931841394354
25 2.70659127776794
26 2.79616357672266
27 2.97716538884947
28 3.10540706991302
29 3.03364674479842
};
\addplot [semithick, color0, opacity=0.3]
table {%
0 3.53496756841957
1 3.56034187986796
2 3.40262732914903
3 3.12040043576985
4 2.88552583796395
5 3.1137579230493
6 3.67439630730181
7 4.40219251039965
8 4.83375417051393
9 5.10671503836854
10 5.39851714206191
11 5.60469927171015
12 5.40417051841031
13 5.04515343249897
14 4.53528449364367
15 4.12448350068549
16 3.53647258659583
17 3.04104635821709
18 2.44967273578677
19 2.37291066719273
20 2.70115695185881
21 3.35877625943297
22 3.77205020156736
23 4.1359008910423
24 4.11818441076248
25 3.71918482457841
26 3.18856037747679
27 2.93524438102415
28 2.84223152088975
29 2.74211676410325
};
\addplot [semithick, color0, opacity=0.3]
table {%
0 3.57723853219815
1 3.64461222088334
2 3.54422972960468
3 3.25335534999685
4 3.01792515943877
5 3.24021075741999
6 3.79533166481725
7 4.2775989696996
8 4.48947022639733
9 4.83603668598167
10 5.15140580824879
11 5.30613266090862
12 5.28016493118252
13 5.09575168745022
14 4.85165643195846
15 4.49776177376517
16 3.97332604828076
17 3.53650837478922
18 3.03860544288437
19 2.59852019065673
20 2.33839654529921
21 2.24734855205693
22 2.30470256670445
23 2.46683530000033
24 2.70187193117278
25 2.91749507634543
26 3.177016513719
27 3.39789017816101
28 3.58257825779772
29 3.70075382299488
};
\addplot [semithick, color0, opacity=0.3]
table {%
0 3.45788150351057
1 3.58260928347073
2 3.55040424469944
3 3.14987196647987
4 2.87388247671143
5 3.20378615967059
6 3.81319001589523
7 4.31885196784951
8 4.71369307129097
9 4.95035073572447
10 5.12625449058206
11 5.1774700412903
12 5.11415568495357
13 4.83054457929057
14 4.35535369769227
15 3.86398803332505
16 3.11979485809499
17 2.66063133985397
18 2.21926426382951
19 1.9276083140064
20 2.03359131031629
21 2.43928492096895
22 2.6361438922939
23 3.03507879723474
24 3.49417298493087
25 3.56864678688882
26 3.38175338508222
27 3.13643408135737
28 2.91989199875588
29 2.81100214629535
};
\addplot [semithick, color0, opacity=0.3]
table {%
0 3.52452840394355
1 3.6273685535714
2 3.59245583826381
3 3.3860817348298
4 3.11939401441888
5 3.37805730359909
6 3.63739594442011
7 4.22811791598782
8 4.6482932763342
9 4.8443751612986
10 4.97310667903284
11 5.01144556212842
12 4.67351456677622
13 4.15877172820943
14 3.56210928315804
15 3.19034088076277
16 2.91609447178834
17 2.78544676508509
18 2.73899893297792
19 2.4211168835752
20 2.41946912111582
21 2.28157613926022
22 2.09267019444061
23 2.0872878666946
24 1.96498115492984
25 1.85535075049173
26 1.82206245246314
27 2.02284756569506
28 2.25494159928231
29 2.42989319404186
};
\addplot [semithick, color0, opacity=0.3]
table {%
0 3.35637863255996
1 3.36216217660825
2 3.34940860800271
3 3.34711210563087
4 3.3266218861233
5 3.74211459011387
6 4.13179184777371
7 4.74267616795271
8 5.01932052516097
9 5.20397403833988
10 5.25709744005045
11 5.22784411783838
12 4.98668500672597
13 4.71367504960847
14 4.28184690905127
15 3.7158716354221
16 2.91836028552944
17 2.38751734587209
18 1.96041879415623
19 1.91084865797238
20 2.09437544295215
21 2.47412454907152
22 2.95033858417615
23 3.3987577804247
24 3.90668933383761
25 4.35528806114354
26 4.85327593235943
27 5.3383424884028
28 5.58403178113307
29 5.53620865125299
};
\addplot [semithick, color0, opacity=0.3]
table {%
0 3.34173262931867
1 3.39616626309407
2 3.45238583701502
3 3.23476082616964
4 3.00699102783686
5 3.34967279483688
6 3.86336478814748
7 4.32007054793967
8 4.70502725844047
9 4.90227876063992
10 5.08207158350405
11 5.27291391989595
12 5.09105195979769
13 4.79832099504562
14 4.44294991036586
15 3.89834945654336
16 3.34362820388035
17 2.63683976854457
18 2.12788623199487
19 1.75141203332049
20 1.86976821981295
21 1.9287453635944
22 1.7411444114892
23 1.64827829401234
24 1.69551007970155
25 1.66688002242658
26 1.76927834413021
27 2.08974137489323
28 2.38001200580064
29 2.6798501432915
};
\addplot [semithick, color0, opacity=0.3]
table {%
0 3.4727565989944
1 3.59212211393626
2 3.55656808566513
3 3.32244351357801
4 3.15066464053262
5 3.47365815672578
6 3.85219171727764
7 4.30027875932756
8 4.67724004291945
9 4.95848367040633
10 5.13177538218669
11 5.07052625763579
12 4.78574740489643
13 4.45350652372691
14 3.97082035719707
15 3.38223761872617
16 2.93920057778572
17 2.52584553779145
18 2.48623929195584
19 2.27287543689205
20 2.17695449254416
21 2.29575022573634
22 2.42593647503975
23 2.65592863610426
24 2.93002477734018
25 3.28057682597
26 3.54660292678242
27 3.50950508560071
28 3.38965374165132
29 3.06332913360303
};
\addplot [semithick, color0, opacity=0.3]
table {%
0 3.5226730614876
1 3.67819535495896
2 3.56064868782486
3 3.37627560537572
4 3.23295205884374
5 3.38168795158182
6 3.7245969299391
7 4.34426243622987
8 4.66094760592777
9 4.80931156708923
10 5.09942708034875
11 5.21864104679499
12 5.05481182732709
13 4.87731353558015
14 4.41416579999151
15 3.84427969182576
16 3.31968479063718
17 2.81163009372428
18 2.43184330684941
19 2.31048236688403
20 2.59259529197681
21 2.83888096320068
22 3.05759249386225
23 3.12223250311312
24 3.09103680948809
25 2.99405654530868
26 2.86369306150339
27 2.8763072204216
28 2.79792095622363
29 2.64884676415549
};
\addplot [semithick, color0, opacity=0.3]
table {%
0 3.39364426181671
1 3.47413328457966
2 3.49362760125915
3 3.24008108035346
4 3.1006712204054
5 3.40197692055845
6 3.82590999308315
7 4.1851766205521
8 4.36664853183473
9 4.3500463297975
10 4.36635043023066
11 4.15733904983708
12 3.6671244674459
13 3.14835163507273
14 2.79866959064448
15 2.89270654720283
16 3.0980365138289
17 3.40975753217359
18 3.43516166921741
19 3.02968585013081
20 2.62011122408992
21 2.24856499412322
22 1.92667716567979
23 1.59181345736477
24 1.10179605246205
25 0.495003527909471
26 0.00510557693512903
27 -0.497628060904772
28 -0.962641228612844
29 -1.34989406804224
};
\addplot [semithick, color0, opacity=0.3]
table {%
0 3.56428910426952
1 3.62753948813066
2 3.6012296674432
3 3.34783056207007
4 3.17139812075359
5 3.38798494095095
6 3.74103799329436
7 4.18804695415637
8 4.50568294184482
9 4.75632990392272
10 4.85227560572255
11 4.76616069931286
12 4.50189105784974
13 4.29203439571891
14 3.87286930701427
15 3.46404535136722
16 2.89090707394049
17 2.96263966312852
18 3.39711335931247
19 3.61507705904507
20 3.83193793655913
21 3.8207033335463
22 3.60536261330908
23 3.3945425319951
24 3.11788370269859
25 2.66156410173256
26 2.16603264545423
27 1.7339041336675
28 1.30880798353469
29 0.829829989876998
};
\end{groupplot}

\begin{groupplot}[group style={group size=1 by 3}]
\nextgroupplot[
xshift=-8,
ylabel={\textcolor{color1}{outer angle}},
ylabel style={font=\large},
xmin=-1.45, xmax=30.45,
ymin=-0.85, ymax=5.85,
width=\figurewidth,
height=\figureheight,
xtick={},
xticklabels={},
axis y line=right,
tick align=outside,
xtick pos=left,
ytick pos=right,
x grid style={white!69.019607843137251!black},
y grid style={white!69.019607843137251!black}
]
\addplot [semithick, color1, opacity=0.3]
table {%
0 2.61950555933346
1 1.91148679239511
2 0.9800599415482
3 -0.217110188560676
4 -0.867938973890784
5 -1.11685381671571
6 -1.20685092292884
7 -1.19612553657888
8 -1.09849275847532
9 -1.22161495066757
10 -1.32089172912551
11 -1.45559669811115
12 -1.5796514358526
13 -1.77294581432246
14 -2.00530639458671
15 -2.33832105154502
16 -2.89903126769385
17 -3.83727763442437
18 -5.18556807874986
19 -6.61730458334486
20 -8.24332283885249
21 -10.0558252037028
22 -11.8572153892428
23 -13.5412363791027
24 -15.0978715384313
25 -16.458287541734
26 -17.5315984062954
27 -18.5145920015132
28 -19.5502557072706
29 -20.583796882955
};
\addplot [semithick, color1, opacity=0.3]
table {%
0 2.70366195954305
1 1.95192946033404
2 1.13611862315948
3 0.0312135857822664
4 -0.455039583803375
5 -0.19343002847393
6 0.210365110981824
7 0.684407858538638
8 1.15116348310388
9 1.40665318043748
10 1.76461633807848
11 2.2135930637623
12 2.6349964010358
13 2.9786465917974
14 3.32315368434731
15 3.86634255199684
16 4.62781252356072
17 5.49054764416003
18 6.45449747792796
19 7.49478543201697
20 8.2139942433306
21 8.69255829975891
22 8.90045843587562
23 8.58642782801775
24 7.88949778944482
25 7.42241221819782
26 6.98744292427548
27 6.61151242161375
28 6.25692265412422
29 5.79436466937483
};
\addplot [semithick, color1, opacity=0.3]
table {%
0 2.70390879274813
1 2.06284230654488
2 1.28751107423576
3 0.274353723261973
4 -0.0865557225496474
5 0.295962518934486
6 0.82939207218058
7 1.61045327291199
8 2.49379316041754
9 3.25239498632427
10 3.90616161022503
11 4.78519522656865
12 5.82762140468566
13 6.89052927723638
14 8.13614108133533
15 9.38969573024471
16 10.2894264871838
17 10.807981771013
18 10.8125222198279
19 10.5091332752195
20 10.0739937923252
21 9.61402070839407
22 9.25898209386927
23 8.84496897556997
24 8.42914294626332
25 7.93971749910984
26 7.40816056071359
27 6.84700900047766
28 6.22201599296404
29 5.62273005197862
};
\addplot [semithick, color1, opacity=0.3]
table {%
0 2.67010882481419
1 1.96971617363226
2 1.0879214302868
3 -0.0250319135090891
4 -0.500412832942605
5 -0.321329141444542
6 -0.00575915189395637
7 0.511539236761362
8 1.1776389592071
9 1.76519461598089
10 2.31720514248705
11 2.91942089619786
12 3.6217733550031
13 4.22682037172477
14 4.92322974999604
15 5.76396485468781
16 6.48248442467833
17 7.27781067245593
18 7.77921595837448
19 7.96555997751913
20 7.67660895670639
21 7.12204355074224
22 6.46216009157125
23 5.86035949037874
24 5.39442329948425
25 4.94720446969553
26 4.49595499649515
27 4.12055658963365
28 3.72112283640161
29 3.46648283097718
};
\addplot [semithick, color1, opacity=0.3]
table {%
0 2.65997650251569
1 1.92589144222464
2 0.921825048974528
3 -0.328802060930487
4 -0.941797019056832
5 -1.15064576742635
6 -1.24325377375617
7 -1.15334418321814
8 -0.898802106032687
9 -0.724402089397287
10 -0.721697429710296
11 -0.865395080713608
12 -0.803854659088975
13 -0.653967499733005
14 -0.496369888803027
15 -0.515904944829673
16 -0.450232923255214
17 -0.530844763160092
18 -0.634495963416866
19 -0.9722508790364
20 -1.49224017170138
21 -2.3135112224469
22 -3.39939413924866
23 -5.04462182538667
24 -6.92053413719749
25 -8.71375229842016
26 -10.1956001471665
27 -11.5487413657754
28 -12.8930749128593
29 -14.2292992635356
};
\addplot [semithick, color1, opacity=0.3]
table {%
0 2.65832762655855
1 1.95238661210138
2 1.07830301722588
3 -0.0809431247682895
4 -0.734380345852921
5 -0.739237205424505
6 -0.364082873522854
7 0.154063570556856
8 0.5007391592552
9 0.558390850601498
10 0.453976559704749
11 0.472280795979543
12 0.412821145954014
13 0.288625904254683
14 0.153289707453371
15 -0.0415383377197749
16 -0.607086688388051
17 -1.24413173763841
18 -2.31036696214161
19 -3.50635170018696
20 -4.94113445818772
21 -6.58017703763813
22 -8.10193501075269
23 -9.38611563014286
24 -10.9232710880828
25 -12.3503827982775
26 -13.6748681506935
27 -14.7720879650724
28 -15.8018972045729
29 -16.8194503971283
};
\addplot [semithick, color1, opacity=0.3]
table {%
0 2.68908658090228
1 1.9866101182228
2 1.02335758240891
3 -0.177687370247217
4 -0.79557846187798
5 -0.969001479273851
6 -0.917666950322799
7 -0.830450243126437
8 -0.660565826748769
9 -0.875583526569837
10 -1.19225680628012
11 -1.53249711665814
12 -1.96980610138735
13 -2.30534583319865
14 -2.66899949140462
15 -3.41463944832244
16 -4.48993518633083
17 -5.86821026229962
18 -7.49339831740616
19 -9.04165624045782
20 -10.3589189050045
21 -11.5126731806801
22 -12.6744354090701
23 -13.597527306352
24 -14.5156369058044
25 -15.434799106369
26 -16.2757645032981
27 -17.0443735435649
28 -18.0466235421681
29 -19.1946845400588
};
\addplot [semithick, color1, opacity=0.3]
table {%
0 2.70034432565367
1 1.91815227713715
2 1.05888452887444
3 -0.128435900420797
4 -0.707089006984893
5 -0.555616737030856
6 -0.266657482988242
7 0.112639927001092
8 0.68383847416667
9 1.09806461418472
10 1.65326427126743
11 2.3600477773853
12 3.07752231796578
13 3.79244572456685
14 4.44813768747766
15 5.02293054344296
16 5.43917563893448
17 5.69975959302294
18 5.49752585962218
19 5.16190514627513
20 4.90355401032716
21 4.71294168545542
22 4.56470658059431
23 4.31529979662424
24 4.18731912641586
25 4.09689233889289
26 4.13737153048105
27 4.17683653372312
28 4.09376298108756
29 4.0049537638829
};
\addplot [semithick, color1, opacity=0.3]
table {%
0 2.71658173713363
1 1.97993606578676
2 1.07751901397388
3 0.11609356817725
4 -0.336880036744819
5 -0.344185543896684
6 -0.077563704627595
7 0.355650008184243
8 0.777087794936465
9 0.939133757315444
10 1.00273952272854
11 1.12232044505616
12 1.19670716682378
13 1.24956744351313
14 1.3397297440672
15 1.40205496292544
16 1.35413185204454
17 1.08656111223944
18 0.676401649997525
19 0.204175465405358
20 -0.30778032875533
21 -0.900318252660627
22 -1.60585835165582
23 -2.6789686645089
24 -4.00113450678989
25 -5.41507036199837
26 -6.99074280913071
27 -8.44735221601767
28 -9.80145240998491
29 -10.9913723532458
};
\addplot [semithick, color1, opacity=0.3]
table {%
0 2.67011013489685
1 1.97662279961282
2 1.11573139660623
3 0.0711341755914727
4 -0.402881776117843
5 -0.1989782886185
6 0.302110175707403
7 0.99096876576559
8 1.64104030426092
9 2.18800614217009
10 2.75915358280556
11 3.20990829065438
12 3.65365791765799
13 4.07640863232632
14 4.55966324150235
15 5.01564077151604
16 5.85745142017754
17 6.65866178264024
18 7.39148105236416
19 7.83732601560301
20 8.00187674086911
21 7.60222373816667
22 6.92283403916472
23 6.38303232214282
24 5.91993563250916
25 5.52394252590441
26 5.27432482671008
27 4.98478174538813
28 4.73997978500852
29 4.56490030171607
};
\addplot [semithick, color1, opacity=0.3]
table {%
0 2.69931929891135
1 2.04327575440857
2 1.09729020147018
3 -0.130440371583397
4 -0.76392456946169
5 -0.829068728739642
6 -0.882218723737957
7 -0.744449530429421
8 -0.733747008773348
9 -0.878547239524565
10 -1.13799505491403
11 -1.34777790980008
12 -1.46368752430491
13 -1.49869743069785
14 -1.51385041001301
15 -1.64547070088193
16 -2.02189197246906
17 -2.48246255204929
18 -3.18641781562074
19 -4.32252439575824
20 -5.7961978323028
21 -7.53487752772209
22 -9.09678979624358
23 -10.5469933044745
24 -11.8687666940607
25 -13.2872946492867
26 -14.681018335819
27 -16.0035407055027
28 -17.2380235149141
29 -18.3979798932416
};
\addplot [semithick, color1, opacity=0.3]
table {%
0 2.71874874449566
1 1.90870947692094
2 0.954972179524646
3 -0.241440202594633
4 -0.765009031151694
5 -0.614933063237388
6 -0.341658214281512
7 0.243930380481588
8 0.643599050521889
9 1.02852206978183
10 1.39134238296373
11 1.82886236099631
12 2.35361230654323
13 2.76414987935601
14 3.14953820112423
15 3.35194393332045
16 3.71598993433066
17 3.97912689879375
18 4.28397038361005
19 4.52478922261925
20 4.53250251625193
21 4.38575861350261
22 4.12274965948743
23 3.78166887354183
24 3.401681851434
25 3.15841283838882
26 3.14391584439841
27 3.1437778234799
28 3.21832399970171
29 3.35382486605699
};
\addplot [semithick, color1, opacity=0.3]
table {%
0 2.75939031503598
1 2.02419390432946
2 1.12910421995586
3 0.0166649474640952
4 -0.452526750052577
5 -0.39641378180986
6 -0.188435141521952
7 0.180008571131856
8 0.533395050695045
9 0.735569692174236
10 0.853283158404512
11 0.851429416357581
12 0.816319173688099
13 0.724471184788452
14 0.578533238423789
15 0.285773168182738
16 -0.126936492345934
17 -0.929404443835654
18 -1.77748823884474
19 -2.63580444078069
20 -3.85605839612981
21 -5.59234328959522
22 -7.42151632162512
23 -8.9982374933401
24 -10.8790421129046
25 -12.5758204264116
26 -14.0185931186653
27 -15.3477187434521
28 -16.5013960261498
29 -17.5426094809126
};
\addplot [semithick, color1, opacity=0.3]
table {%
0 2.71924842644924
1 2.03859558637315
2 1.12573213725142
3 -0.0577873701944203
4 -0.515403613313016
5 -0.374351477034669
6 0.102432996574302
7 0.675037602231672
8 1.46041276191885
9 2.03650647418261
10 2.52545065148001
11 3.01667659750414
12 3.69303998753685
13 4.43887373044344
14 5.17188885910687
15 5.87629607419456
16 6.41184350637486
17 7.04032347394163
18 7.3346588140222
19 7.29830891737191
20 6.84778686524645
21 6.10316513983111
22 5.45632235397477
23 4.72050522787223
24 3.92311316591121
25 3.15813176561599
26 2.42390604169781
27 1.64048140264421
28 0.90057636938216
29 0.202120258449025
};
\addplot [semithick, color1, opacity=0.3]
table {%
0 2.65526014053647
1 1.85517483459315
2 0.985685869014805
3 -0.060768320739859
4 -0.540573836473101
5 -0.602864318605002
6 -0.427679343043136
7 -0.123189153001626
8 0.137119806337182
9 0.335130279630519
10 0.537130333751049
11 0.719007462949817
12 0.917113095996545
13 0.920741350461604
14 1.05641545402256
15 1.08949653742901
16 1.06271460623789
17 1.00350667513697
18 0.792430373301746
19 0.61455059555384
20 0.352612621519111
21 0.0325011008008573
22 -0.658464650639983
23 -1.50675721803775
24 -2.73541561082051
25 -3.98611568836952
26 -5.13823546541345
27 -6.14148819671492
28 -6.96672332270359
29 -7.64867611759768
};
\addplot [semithick, color1, opacity=0.3]
table {%
0 2.76336696606541
1 2.04605211759736
2 1.02786002479152
3 -0.0359973006641621
4 -0.459112767449328
5 -0.287424392187367
6 0.0727008898271713
7 0.524211176053537
8 1.0885444316172
9 1.58424093945323
10 2.17209992259071
11 2.70792207166001
12 3.20108736791907
13 3.74362976203599
14 4.23575198072281
15 4.72020569340462
16 5.3364484112357
17 6.02154318326474
18 6.44638032474696
19 6.42995117657615
20 6.1313117455974
21 5.43093535800986
22 4.4944482532858
23 3.38758201666803
24 2.27995354591862
25 1.1468287382976
26 0.0543549874340847
27 -1.20005218886987
28 -2.73492729243505
29 -4.34575578800237
};
\addplot [semithick, color1, opacity=0.3]
table {%
0 2.6438696788416
1 1.95494662805965
2 1.17874477997851
3 0.0107602224075478
4 -0.463510649136339
5 -0.323440218797318
6 0.116731175300474
7 0.754523879879287
8 1.55384531824679
9 2.2155320612566
10 2.82578068937977
11 3.16096220508723
12 3.67303834627354
13 4.131189822515
14 4.51856659472794
15 4.72992695315545
16 5.09234551785523
17 5.21860938463463
18 5.12380442440485
19 4.68664936932345
20 4.28495452039381
21 3.82337198871203
22 3.36038806928208
23 3.00120156772647
24 2.62995224415271
25 2.54105382067012
26 2.62378542291716
27 2.99984559541183
28 3.30169102922334
29 3.62184572941589
};
\addplot [semithick, color1, opacity=0.3]
table {%
0 2.60653024531803
1 1.94080048573905
2 1.07585814963554
3 -0.0481287829233601
4 -0.371718423155386
5 -0.251021824958604
6 0.165533111831325
7 0.714843105377374
8 1.24074103923867
9 1.78050077178606
10 2.28654031234596
11 2.85900041753506
12 3.53818415057052
13 4.13194412766205
14 4.82694058388631
15 5.56671943100244
16 6.42719836421484
17 7.45814790364078
18 8.42231558974862
19 9.08108824470672
20 9.51499401233623
21 9.55434040822239
22 9.39430276939061
23 9.01285134442753
24 8.66073440326231
25 8.25775116797665
26 7.91042985220174
27 7.47662214581804
28 7.07999407809354
29 6.64574289250792
};
\addplot [semithick, color1, opacity=0.3]
table {%
0 2.67183990042016
1 1.84370965436382
2 0.814246429200148
3 -0.411152003290594
4 -1.05639214215467
5 -1.25414290380762
6 -1.32455753618744
7 -1.15989931597173
8 -0.997192006612343
9 -0.968623119947724
10 -1.2577889237272
11 -1.90044949309599
12 -2.57546469449507
13 -3.45840878758611
14 -4.63175376961487
15 -6.22615138200982
16 -7.85049837504954
17 -9.57761740953963
18 -11.3150617451513
19 -12.9138874361152
20 -14.2252982996066
21 -15.7402960554981
22 -17.1584445471529
23 -18.501767202864
24 -19.9109911634331
25 -21.3078082794771
26 -22.6189582349959
27 -23.921268412845
28 -25.3697199200122
29 -26.7141143229504
};
\addplot [semithick, color1, opacity=0.3]
table {%
0 2.65664401364741
1 1.84253305646656
2 0.921420455390553
3 -0.25903913630545
4 -0.772184237165224
5 -0.840837594589338
6 -0.527949977445145
7 -0.144856361747088
8 0.167201999690958
9 0.129355763124455
10 0.047970005733605
11 -0.202195256439902
12 -0.342032272588746
13 -0.733005464283316
14 -1.44160400367792
15 -2.39128611581866
16 -3.59769911076977
17 -5.32798514697426
18 -6.93319997465418
19 -8.47033027154955
20 -9.82201969515057
21 -11.1860119142424
22 -12.5159229128398
23 -13.884492995388
24 -15.2610479716388
25 -16.7085803799235
26 -17.9812851650804
27 -19.2564423545319
28 -20.5174624298462
29 -21.9691376049799
};
\end{groupplot}

\begin{groupplot}[group style={group size=1 by 3}]
\nextgroupplot[
xshift=-8,
xmin=-1.45, xmax=30.45,
ymin=2.7, ymax=6.7,
width=\figurewidth,
height=\figureheight,
xtick={},
xticklabels={},
yticklabels={},
tick align=outside,
tick pos=left,
x grid style={white!69.019607843137251!black},
y grid style={white!69.019607843137251!black}
]
\addplot [line width=0.06pt, color0, mark=*, mark size=2, mark options={solid,draw=black}]
table {%
0 3.31996634253658
1 3.45443899460193
2 3.38784218387077
3 3.01931286439371
4 2.82906626173755
5 3.09427938765557
6 3.60416870184349
7 4.24596487007442
8 4.84338888587772
9 5.27994908427636
10 5.61004074039071
11 5.90268352537916
12 6.05852129333431
13 6.16858387553312
14 6.19509636026208
15 6.21485180933973
16 6.20378189365436
17 6.1468591562609
18 6.14787992255152
19 6.14579317317396
20 6.15283082950704
21 6.15412613868876
22 6.14366281427887
23 6.16587792193215
24 6.18223254289368
25 6.18638821201769
26 6.14794417270148
27 6.14179954980725
28 6.15812095860932
29 6.16746194810668
};
\end{groupplot}

\begin{groupplot}[group style={group size=1 by 3}]
\nextgroupplot[
xshift=-8,
xmin=-1.45, xmax=30.45,
ymin=-0.85, ymax=5.85,
width=\figurewidth,
height=\figureheight,
xtick={},
xticklabels={},
yticklabels={},
axis y line=right,
tick align=outside,
xtick pos=left,
ytick pos=right,
x grid style={white!69.019607843137251!black},
y grid style={white!69.019607843137251!black}
]
\addplot [line width=0.06pt, color1, mark=*, mark size=2, mark options={solid,draw=black}]
table {%
0 2.65103446372252
1 1.87298481713709
2 1.03310235020523
3 -0.0349224785257646
4 -0.681923979276541
5 -0.614035490335335
6 -0.208100847346677
7 0.33428430837777
8 0.710486243049944
9 0.726233644866842
10 0.520411660737353
11 0.347599665643602
12 0.244300607278545
13 0.195112904269273
14 0.20629800498181
15 0.161911176310666
16 0.161283251423433
17 0.247899352697984
18 0.208651205023874
19 0.171253015388636
20 0.20029198108343
21 0.172890109571832
22 0.187770311286831
23 0.213147053788955
24 0.185796243819713
25 0.165625930691843
26 0.187584184388062
27 0.20252014981221
28 0.179459395114634
29 0.2013127196102
};
\end{groupplot}
