# Supplementary material for: Identification of Gaussian Process State Space Models
Source: arXiv:1705.10888 source file (2017-11-07)
Supplement: Supplementary file 2 [file tikz_samples_ep-2-all.tex]

\definecolor{color0}{rgb}{0.12156862745098,0.466666666666667,0.705882352941177}
\definecolor{color1}{rgb}{1,0.498039215686275,0.0549019607843137}

\begin{groupplot}[group style={group size=1 by 3}]
\nextgroupplot[
xshift=-8,
title={2 episodes},
title style={font=\large},
ylabel={\textcolor{color0}{inner angle}},
ylabel style={font=\large},
xmin=-1.45, xmax=30.45,
ymin=2.7, ymax=6.7,
width=\figurewidth,
height=\figureheight,
xtick={},
xticklabels={},
tick align=outside,
tick pos=left,
x grid style={white!69.019607843137251!black},
y grid style={white!69.019607843137251!black}
]
\addplot [semithick, color0, opacity=0.3]
table {%
0 3.41289310163331
1 3.05051687853909
2 3.09932099612203
3 3.18769350278898
4 3.24552780666672
5 3.16750664224544
6 3.00911921170606
7 2.77901212901609
8 3.0379600792271
9 3.37765183287035
10 3.61249801177389
11 4.09212460456359
12 4.49405002386523
13 4.89425079130043
14 5.14834302592042
15 5.22811732691164
16 5.1709354410081
17 5.20652795110208
18 5.29609598327113
19 5.08648505446709
20 5.15643644452188
21 5.20950239927538
22 5.13170088578445
23 5.2139785755416
24 5.25817689210719
25 5.29775693994264
26 5.34611319746027
27 5.55754004293797
28 5.70258893992972
29 5.62892835404119
};
\addplot [semithick, color0, opacity=0.3]
table {%
0 3.62675117947097
1 3.30438159022828
2 3.24496304542662
3 3.15831259869557
4 2.85631320277671
5 2.72961164148492
6 2.59719963915924
7 2.13877549047287
8 2.1917911773713
9 2.32262268464628
10 2.27705974013039
11 2.49243116370972
12 2.94868424780364
13 3.19410479407622
14 3.43685232435551
15 3.79737713322084
16 4.03431545575104
17 4.0524222547038
18 4.03441281886615
19 4.02117971725268
20 3.96018349781977
21 4.1388030388022
22 4.10861723799349
23 4.10230030947739
24 4.28815427295851
25 4.24343432586917
26 4.30048799706524
27 4.2675985212859
28 4.29603386662686
29 4.29772959282216
};
\addplot [semithick, color0, opacity=0.3]
table {%
0 3.51920735780842
1 3.48691390425132
2 3.38983396189592
3 3.23430553727682
4 3.07195134039274
5 3.17285105888252
6 3.44767391806781
7 3.34321895047491
8 3.47420585899804
9 3.57065838086876
10 3.72594495414718
11 4.02819338560428
12 4.63758033404928
13 4.89284830350272
14 5.16048716835963
15 5.03660601788048
16 5.11990922347906
17 5.1152404713927
18 5.06110089302616
19 5.07143687783987
20 4.88036080709466
21 4.75699423161772
22 4.76174232666134
23 4.61760263230762
24 4.51985382243341
25 4.47649833095254
26 4.31614150761705
27 4.20984454305424
28 4.02773055713415
29 3.96065949201223
};
\addplot [semithick, color0, opacity=0.3]
table {%
0 3.45386092242128
1 3.48785816760023
2 3.44484026463111
3 3.21473825385762
4 2.73305974499629
5 2.819741822446
6 2.68993416948298
7 2.30989830657704
8 2.6970870435561
9 2.9336500451896
10 3.33888358594897
11 3.44512235018261
12 3.97707432925544
13 4.45961698016017
14 4.82666939252971
15 4.91836188817522
16 5.1288635742437
17 5.40367778775085
18 5.44210086249605
19 5.53934750436078
20 5.71085602216982
21 5.96716459913452
22 6.14952249689501
23 6.26049630026405
24 6.4379299483277
25 6.53000985960386
26 6.57251006607482
27 6.54923969186839
28 6.57789931997358
29 6.62262525518004
};
\addplot [semithick, color0, opacity=0.3]
table {%
0 3.75113967083616
1 3.61013021652081
2 3.51511750035992
3 3.6352489190781
4 2.9288019592271
5 2.71047392138709
6 2.63220810993761
7 2.35053094452881
8 2.8951364671782
9 3.31474634035035
10 3.84407996221008
11 4.15211989754515
12 4.65558302176165
13 4.81871414123971
14 5.23283362574843
15 5.46633245126215
16 5.47059267939886
17 5.63130262688719
18 5.92271451286946
19 5.85545826806387
20 6.05301380313106
21 6.12016000672075
22 6.11549902050237
23 6.28455490703889
24 6.34619483358154
25 6.43365538139582
26 6.40105305527574
27 6.55481521126226
28 6.49068321460378
29 6.60511535174508
};
\addplot [semithick, color0, opacity=0.3]
table {%
0 3.65425466628332
1 3.52933030260276
2 3.63854288748125
3 3.36048177474356
4 2.99586141430448
5 2.71308591585516
6 2.51689930622233
7 2.25277023941729
8 2.5335158555683
9 2.68839888870116
10 2.6609162967361
11 2.58616625855091
12 3.05272820594346
13 3.12309426329273
14 3.2121808590703
15 3.07552727748617
16 2.9189785356645
17 2.82291399280707
18 2.82351125927817
19 2.74825638727305
20 2.61597433227212
21 2.56675260427609
22 2.48256851956328
23 2.46553050473178
24 2.37180397660978
25 2.29850864495608
26 2.2334323668424
27 2.17046102821872
28 2.10337310441086
29 2.1309345218947
};
\addplot [semithick, color0, opacity=0.3]
table {%
0 3.47926468719603
1 3.25104162179219
2 3.12331942759417
3 3.31832333465087
4 2.94850105584201
5 2.97739610730939
6 2.85491275374917
7 2.45571927373938
8 2.52720037774265
9 2.67712432215892
10 2.92913178536277
11 3.02802391355047
12 3.44189203898254
13 3.72892684726738
14 4.03901785699453
15 4.13560475231204
16 3.95051918917776
17 3.82133170011931
18 3.79497283342966
19 3.81401651248842
20 3.65929781046563
21 3.69401958553862
22 3.56464296376372
23 3.6418027433405
24 3.72784778863905
25 3.87012879308984
26 3.74206355069309
27 3.79525027576085
28 3.76613662852949
29 3.85794307688957
};
\addplot [semithick, color0, opacity=0.3]
table {%
0 3.18055302886721
1 3.13405225361342
2 3.31943398626576
3 3.40561337021024
4 3.31991724794387
5 3.54017251988422
6 3.31855795141351
7 2.9163178492169
8 3.24182363582723
9 3.82304993816413
10 4.01161796692156
11 4.16212845570058
12 4.48454829881319
13 4.64014697573353
14 4.89345224049462
15 4.87437809490021
16 4.88425309973117
17 4.98319576839412
18 5.10688083987627
19 5.14791330110702
20 5.2798077644698
21 5.27085163391758
22 5.14119621408158
23 5.23897893884893
24 5.18564980714668
25 5.2648594980428
26 5.30413762428235
27 5.39436393026073
28 5.36850351397679
29 5.3100243340421
};
\addplot [semithick, color0, opacity=0.3]
table {%
0 3.5579296617354
1 3.5689905343398
2 3.63687483813142
3 3.37876340664492
4 2.98807306346975
5 2.93629666198573
6 2.75841349294657
7 2.33796891452453
8 2.47656697418567
9 2.7721244036664
10 2.92285009575676
11 2.95793833906682
12 3.2724550962092
13 3.65385482216081
14 3.89241309165458
15 3.96795709997901
16 3.93319143713262
17 3.80350124431383
18 3.83111685328305
19 3.72165334252428
20 3.67886543022167
21 3.4499539204686
22 3.31176369587767
23 3.24844369598971
24 3.32401795248082
25 3.31585534230585
26 3.14794509376642
27 3.10664300935888
28 3.0995864125112
29 3.02574863326737
};
\addplot [semithick, color0, opacity=0.3]
table {%
0 3.44873839294622
1 3.37770145945011
2 3.15420234412274
3 3.01515415823868
4 2.55935031559012
5 2.33017306496655
6 2.14394942620106
7 1.82476887072867
8 2.01764420117516
9 2.29427807053407
10 2.61501821669817
11 2.93057825880766
12 3.16621714430747
13 3.29459566726943
14 3.40321102904514
15 3.3622237556343
16 3.25090869586216
17 3.28752186836531
18 3.46725346483945
19 3.29755865648523
20 3.1980836075574
21 3.28721380283712
22 3.2833563967269
23 3.18687777178133
24 3.13036299876715
25 3.09884306764517
26 3.11052897217013
27 3.03286822695524
28 2.96884439001992
29 2.97808586553909
};
\addplot [semithick, color0, opacity=0.3]
table {%
0 3.58420164627459
1 3.56315172847734
2 3.64422783393182
3 3.56908436746244
4 3.1676671523747
5 3.29502773115027
6 3.18100256178842
7 3.11709712220186
8 3.41142009774581
9 3.71009787876651
10 3.95164082104152
11 4.03041507918881
12 4.49453722306205
13 5.07429942414232
14 5.54146379230816
15 5.82293931536836
16 5.80643435364313
17 5.69136909598622
18 5.6015705945571
19 5.69833808867281
20 5.52783121780868
21 5.52788003684648
22 5.49253398790466
23 5.42866232007745
24 5.54844973899828
25 5.49018686550279
26 5.35912565105571
27 5.16956051847261
28 5.09456279495788
29 5.00543042866399
};
\addplot [semithick, color0, opacity=0.3]
table {%
0 3.78448160283413
1 3.57543583331358
2 3.59729187969974
3 3.51355023652996
4 3.17622273069857
5 3.1609219490948
6 2.96222372609489
7 2.55688092342085
8 2.89796638695417
9 3.33488056487879
10 3.6130526125903
11 3.75940263216863
12 4.15746034119415
13 4.4575144615604
14 4.57248453857018
15 4.66444679395009
16 4.85702339423463
17 4.80699040215944
18 4.83476414752294
19 5.05570705876371
20 5.00215479213775
21 5.03038497096954
22 5.19468029399138
23 5.16030938882612
24 5.24934701625999
25 5.27982649639944
26 5.36577315780855
27 5.23047785763323
28 5.26439741567414
29 5.35723917567154
};
\addplot [semithick, color0, opacity=0.3]
table {%
0 3.50896874149356
1 3.08184782933726
2 2.88331324877944
3 2.63132424333118
4 2.37192298813664
5 2.32581503732485
6 2.2460852425436
7 2.16290459580621
8 2.30610429067988
9 2.67384441830331
10 2.80743506375509
11 2.95234414286827
12 3.52092328635497
13 3.86845687376568
14 4.35746502702342
15 4.17016070403898
16 4.03326566191116
17 3.85515004157744
18 3.55650054259544
19 3.17237454728917
20 2.9840264332989
21 2.84833868096806
22 2.61658382923273
23 2.63755145291391
24 2.59700770234444
25 2.44036159809733
26 2.34772037747675
27 2.35593248654693
28 2.24796941278073
29 2.1122190650888
};
\addplot [semithick, color0, opacity=0.3]
table {%
0 3.37903160453369
1 3.34791338095471
2 3.21253666599565
3 2.8364156535121
4 2.79741837440454
5 2.6531941367424
6 2.66088530772564
7 2.64736997555185
8 2.9940322683173
9 3.41194804001864
10 3.53639039460047
11 3.66212458478583
12 4.09033011211297
13 4.27641100484995
14 4.53066665938552
15 4.36229463703081
16 4.0413710243163
17 3.71032759951987
18 3.38683720338181
19 3.13093188213943
20 2.84267286244253
21 2.5575011903187
22 2.33113118809841
23 2.09602902373151
24 2.00087831417838
25 1.80821756218347
26 1.46570008919404
27 1.17524758761581
28 0.929503033255491
29 0.605402801973965
};
\addplot [semithick, color0, opacity=0.3]
table {%
0 3.63352026726901
1 3.59284484400665
2 3.49960555564545
3 3.31117996451623
4 2.80743576720903
5 2.90449073097887
6 2.66469669683802
7 2.63760924593396
8 3.04905738018359
9 3.21031678152213
10 3.25900042058241
11 3.37787760294867
12 3.87621614616002
13 4.1516636503025
14 4.39092933046316
15 4.4433262899484
16 4.40098881970106
17 4.28812303357948
18 4.29506434212242
19 4.30067896720977
20 4.27119544766952
21 4.28425698986412
22 4.3639117856862
23 4.40439327282304
24 4.5002550120115
25 4.66360158074249
26 4.71968746569307
27 4.8169522443589
28 4.87683389196641
29 4.97113800416688
};
\addplot [semithick, color0, opacity=0.3]
table {%
0 3.52660760083237
1 3.37595425791963
2 3.31513279183825
3 3.19482915292183
4 3.11199098191601
5 3.17867527795835
6 3.26195850862421
7 3.17300992301324
8 3.40505346497058
9 3.67022830442675
10 4.01426209864774
11 4.04499262788198
12 4.57885893004965
13 4.69046269466621
14 4.88611083746756
15 4.82120058358255
16 4.76931829117432
17 4.49991172844968
18 4.17454188200033
19 3.94698551680106
20 3.75445801218215
21 3.55549477475807
22 3.43215256050371
23 3.20695579216881
24 3.06632330246036
25 2.92187387645647
26 2.9270352417562
27 2.65328228294354
28 2.63271831102881
29 2.64100940007448
};
\addplot [semithick, color0, opacity=0.3]
table {%
0 3.76207290852536
1 3.73728978376529
2 3.49985425744116
3 3.4440824291077
4 3.01449563479132
5 2.99246394771615
6 2.76974579776704
7 2.18560805697497
8 2.55959273294485
9 2.66550449477737
10 2.99249281909692
11 3.14010190160737
12 3.60326320926003
13 3.93246371796845
14 4.29307222293505
15 4.40152011396058
16 4.45851644815144
17 4.6184567377893
18 4.65899347584473
19 4.65120844835968
20 4.65132583622642
21 4.76590746714972
22 4.84289738979881
23 5.03472381739981
24 5.1714487725008
25 5.15761121976826
26 5.13343910943851
27 5.30488068931868
28 5.35857108376541
29 5.31978249292032
};
\addplot [semithick, color0, opacity=0.3]
table {%
0 3.47792189592837
1 3.61059092176214
2 3.72327987498364
3 3.58796219866349
4 2.94904056420882
5 2.92249459157107
6 2.48135833150399
7 2.16963953105363
8 2.59223045008482
9 2.894751870194
10 3.29037824253779
11 3.389674905328
12 3.79154397780932
13 3.82566129133623
14 4.02598480306737
15 3.93692668193681
16 3.82781205056498
17 3.6415181762927
18 3.30255725365307
19 3.17246326400874
20 2.90200189317053
21 2.7787525375912
22 2.74729498138522
23 2.49734659802284
24 2.58508777745006
25 2.48306683134125
26 2.44746402609748
27 2.26562133283082
28 2.14332005753292
29 2.12420892469049
};
\addplot [semithick, color0, opacity=0.3]
table {%
0 3.52731888958683
1 3.28265758936634
2 3.13792883733901
3 3.01988751027391
4 2.69605161897985
5 2.50763670457837
6 1.91889145798881
7 1.41973380349385
8 1.69473385768298
9 2.11818759639376
10 2.32250137386641
11 2.6325720266764
12 3.20346326230072
13 3.59858669233028
14 4.03874862953272
15 4.36950721483386
16 4.31469390242844
17 4.47352781465091
18 4.67637574129423
19 4.9119721495136
20 4.96941453584157
21 4.94920019497943
22 5.09296616934162
23 5.09690641447952
24 4.94328929880438
25 4.85741585817567
26 4.89121338094728
27 4.93530665602228
28 4.85582632465361
29 4.81999110735648
};
\addplot [semithick, color0, opacity=0.3]
table {%
0 3.57710055848102
1 3.39083371735406
2 3.41994549868665
3 3.19117139248922
4 2.87425345933613
5 2.74638737395543
6 2.47930868670814
7 1.7785974742086
8 1.71487960220785
9 1.55716952684092
10 1.81538144662967
11 1.99027400823401
12 2.46528141889312
13 2.50776971779713
14 2.80492421425351
15 2.74509679498134
16 2.54119904229191
17 2.42856615815067
18 2.2323594611436
19 2.06158823520603
20 1.80839644204182
21 1.86482721922895
22 1.76970641540005
23 1.57871017639856
24 1.57331862925958
25 1.53151809843888
26 1.55428275133155
27 1.5740974917409
28 1.60028775334599
29 1.60465494260825
};
\end{groupplot}

\begin{groupplot}[group style={group size=1 by 3}]
\nextgroupplot[
xshift=-8,
xmin=-1.45, xmax=30.45,
ymin=-0.85, ymax=5.85,
width=\figurewidth,
height=\figureheight,
xtick={},
xticklabels={},
yticklabels={},
axis y line=right,
tick align=outside,
xtick pos=left,
ytick pos=right,
x grid style={white!69.019607843137251!black},
y grid style={white!69.019607843137251!black}
]
\addplot [semithick, color1, opacity=0.3]
table {%
0 1.94549092899313
1 1.37177223531952
2 0.412717598122349
3 -0.523252845725859
4 -0.243139010335787
5 0.188910096735247
6 1.06091144148161
7 2.37064404878736
8 3.38744937047385
9 3.920869110506
10 4.42517324786769
11 4.79401740816412
12 4.50002150162083
13 3.82784008234888
14 3.0988845678135
15 2.17659858293533
16 1.7126988508748
17 1.56636219204187
18 0.92529232179119
19 0.436160068106805
20 0.226780826664505
21 -0.389839304251671
22 -0.665198732354115
23 -1.06572580829257
24 -1.69103895793317
25 -2.3080142210969
26 -2.74518868755263
27 -3.06456054982019
28 -3.51578894217637
29 -4.04899035429859
};
\addplot [semithick, color1, opacity=0.3]
table {%
0 2.84687027260119
1 2.288118242207
2 1.45845994451595
3 0.839253205234309
4 0.744946252032781
5 0.93673565430066
6 1.75038498943345
7 3.16648804293795
8 4.21291333868069
9 5.2424427766175
10 5.31921629165915
11 5.79204465073737
12 5.99140157887772
13 5.90991341132755
14 5.66866571980713
15 5.23140954883776
16 4.50815458565231
17 4.18628913719635
18 3.80816122895569
19 3.40331413195662
20 3.32329458280975
21 2.72523665246598
22 2.27478176635914
23 1.8181953573383
24 1.19158659757106
25 0.339940101734422
26 -0.493278287122497
27 -0.761851562539364
28 -1.44870833403248
29 -2.07136265021478
};
\addplot [semithick, color1, opacity=0.3]
table {%
0 2.69508830974404
1 1.70091722022634
2 0.791696450288661
3 -0.150633115074564
4 0.0626785859429422
5 0.237994914266014
6 0.522864534539394
7 1.59826279047895
8 2.28852757056264
9 3.27929515463339
10 3.60978886372121
11 3.5762060702587
12 3.68134143197285
13 3.49114826756662
14 3.47753322503737
15 3.33553900354105
16 2.82939077289031
17 2.11269131167194
18 1.43121624135182
19 1.04451534088733
20 0.610706588927771
21 0.312199690140952
22 -0.157197810366569
23 -0.752585182974636
24 -1.05119142833877
25 -1.46717877129575
26 -1.8598432656766
27 -2.66899150956853
28 -3.08763403066465
29 -3.60649807707768
};
\addplot [semithick, color1, opacity=0.3]
table {%
0 2.69230092314131
1 2.56486346598884
2 2.11093246068557
3 1.70531743438374
4 1.86688702467328
5 1.85763881920301
6 2.36606673513379
7 3.43361807303447
8 4.27544041185034
9 4.53439990586508
10 4.67287957319237
11 5.7115009987293
12 5.12465972976976
13 4.44230858938624
14 3.54177204012692
15 3.13207209085047
16 2.571956254758
17 2.22084332611218
18 1.7711524415123
19 1.80966841667274
20 1.89715792032971
21 1.87342249158379
22 1.90729155820859
23 1.70826821743243
24 1.26216297737045
25 0.859086622424631
26 1.0004421500603
27 1.31271935306676
28 1.56458163296335
29 1.57548400705722
};
\addplot [semithick, color1, opacity=0.3]
table {%
0 1.77451900689785
1 0.862401505050924
2 -0.220266948357239
3 -1.18175572523456
4 -1.41623852353719
5 -1.13008055305302
6 -1.06225939527273
7 -0.481330285096492
8 0.388285922702984
9 1.09883724030976
10 1.54360742756199
11 1.88449813935754
12 1.42717395957824
13 1.38421633653801
14 0.461112796072094
15 -0.19681057481526
16 -0.611038748135121
17 -0.950241234587875
18 -1.52717566820953
19 -1.67692023517892
20 -2.08086091704153
21 -2.39716652215811
22 -2.81838463732152
23 -3.42292691011127
24 -4.01703653618905
25 -4.66480511679705
26 -5.21532018527776
27 -5.83663196447709
28 -6.40744848888199
29 -7.07474232021871
};
\addplot [semithick, color1, opacity=0.3]
table {%
0 2.71596271260996
1 1.70788152860271
2 0.710406389485083
3 -0.11731980101106
4 -0.215330133240434
5 -0.45222473890032
6 -0.0466179643478863
7 0.487831709271797
8 1.23350793860979
9 2.02633481529244
10 2.36488702147274
11 2.88219840502784
12 2.59114812832771
13 2.17580152690233
14 1.5728483063935
15 1.07541171620259
16 0.2483964844394
17 -0.0859944006870084
18 -0.753629884821363
19 -1.33483716087173
20 -1.69526454150128
21 -2.12487618822936
22 -2.60912103362679
23 -3.02590418833541
24 -3.94857366577763
25 -4.83047585845764
26 -5.37602580857545
27 -5.98852132574754
28 -6.51619699113763
29 -7.40708497492976
};
\addplot [semithick, color1, opacity=0.3]
table {%
0 2.54671592861176
1 2.06054097777691
2 0.512673924139882
3 -0.286398885747877
4 -0.130494844085645
5 0.171789055945121
6 0.608342400239675
7 1.41516656828755
8 1.95274218538215
9 2.06324885167157
10 2.35003909989709
11 2.58426672781206
12 2.33840850110493
13 1.88413759681775
14 1.29481524382834
15 0.609431670139619
16 -0.252143381958623
17 -1.22079545988178
18 -2.09653714236772
19 -2.68875011729857
20 -3.68542509227806
21 -4.38473798877582
22 -5.0678211153084
23 -5.88892917652605
24 -6.74549449332986
25 -7.73479875122551
26 -8.64236593535736
27 -9.703605776425
28 -10.7733944682924
29 -11.9116616069673
};
\addplot [semithick, color1, opacity=0.3]
table {%
0 2.67118869304877
1 1.83753894171216
2 0.607510421824559
3 -0.388789476691997
4 -0.15044557208733
5 -0.192546975079857
6 0.358821773446499
7 1.33364397480292
8 1.8817752254605
9 2.53439759875412
10 2.89488231627589
11 3.38181482622037
12 3.28375266891966
13 3.16729619192449
14 2.91333078147511
15 2.96579842208352
16 2.71820543273191
17 2.91488969861856
18 2.87880397926511
19 2.77806129418871
20 2.95268356567587
21 3.08049977971707
22 3.20616249712534
23 3.53314834578866
24 3.94567769550544
25 4.15392934959092
26 4.17576947728335
27 4.5780236257267
28 4.78984387188506
29 4.93497796678828
};
\addplot [semithick, color1, opacity=0.3]
table {%
0 2.45947585557125
1 1.63853409511091
2 0.640296462113346
3 -0.100054699815461
4 0.114813968291017
5 0.395637923379864
6 1.42175067908173
7 2.61234393940969
8 3.35650835973777
9 3.91859843460002
10 4.04370809725658
11 4.46921656162688
12 4.24661160692368
13 3.7467628433151
14 2.88093589617227
15 2.04912570211525
16 1.37013216934515
17 1.0162202287984
18 0.514169331604135
19 -0.0336534922078489
20 -0.539624068984248
21 -0.875394080936944
22 -1.34664841763573
23 -1.49545493024725
24 -2.07182087590276
25 -2.6102519522664
26 -3.24895503796615
27 -3.67310752400727
28 -4.31560377202445
29 -5.09946364826232
};
\addplot [semithick, color1, opacity=0.3]
table {%
0 2.49702527979295
1 2.05009011998423
2 0.889846155399146
3 0.0582686712932183
4 -0.0113720555080032
5 0.0685438951508104
6 0.331914989689293
7 0.966230425781768
8 1.63049104911505
9 2.0434105411191
10 1.83368446585219
11 1.55910749509825
12 0.91021337569069
13 0.414143825197426
14 -0.63758147813299
15 -1.45240935578932
16 -2.32017074945537
17 -3.31657282571002
18 -4.42570517310707
19 -5.3869070467823
20 -6.46844850966612
21 -7.63238660826853
22 -8.70352906713266
23 -9.70350171282728
24 -10.6380000157036
25 -11.7574410541693
26 -12.800707017022
27 -13.9311477323909
28 -14.9655041557577
29 -16.025908899447
};
\addplot [semithick, color1, opacity=0.3]
table {%
0 2.70298495124686
1 2.19091409279405
2 0.846818266945375
3 -0.144098146873482
4 -0.199969088259067
5 -0.118235055831022
6 -0.00459135412549827
7 0.502843039813873
8 1.60894786401401
9 2.32401101575662
10 2.94212746948758
11 3.19065442065359
12 2.90890350352211
13 2.53289929512278
14 1.66531106016028
15 0.654811721064792
16 0.0224003458941837
17 -0.622556708566231
18 -1.29121840030001
19 -1.93424667169132
20 -2.36140679577779
21 -3.23365485755812
22 -3.69846429318353
23 -4.26445358658943
24 -5.02261113193519
25 -5.80373628325836
26 -6.0849627866531
27 -6.46496395391233
28 -7.09586699699206
29 -7.70643273002027
};
\addplot [semithick, color1, opacity=0.3]
table {%
0 2.41266196250574
1 1.68881885527506
2 0.920641378713913
3 0.205290632368779
4 0.476259697848308
5 0.394898784335377
6 0.529146744064716
7 1.27253952840538
8 2.05184277062962
9 2.59092072238814
10 2.80741922485377
11 3.18639388907344
12 3.19657610420445
13 3.1484917911609
14 2.90339036989602
15 2.93188133153763
16 2.52571206133937
17 2.59689398008367
18 2.34545069964998
19 2.32221856330443
20 2.29257754886331
21 2.22099142792132
22 2.16594649775422
23 1.92062830770661
24 1.79078031801938
25 1.93301509450337
26 1.87926355292309
27 1.43966695433823
28 1.28349449117789
29 1.26077189026528
};
\addplot [semithick, color1, opacity=0.3]
table {%
0 2.61708714695282
1 2.6039888575128
2 1.38189282020365
3 0.54759363997664
4 0.396223588833246
5 0.60395701433689
6 1.27907661769211
7 2.33046223416323
8 3.52019030481296
9 4.44395003708997
10 4.91615020160898
11 5.39973855653283
12 5.04366345701147
13 4.79671442387463
14 3.96166280586158
15 3.51298384902709
16 2.93914756810941
17 2.23067968191719
18 1.56631792836957
19 1.15745371430301
20 0.526188636157793
21 0.00468461526536146
22 -0.470892843081955
23 -0.997902933570799
24 -1.43408610086183
25 -1.88221669141607
26 -2.47120631467357
27 -3.33786866881699
28 -3.99664620340802
29 -4.47618063159133
};
\addplot [semithick, color1, opacity=0.3]
table {%
0 2.21879099613857
1 1.6154299270273
2 0.600883987963034
3 -0.256130589906091
4 -0.641966870389455
5 -0.545012423392697
6 -0.290997733915841
7 0.941986997629682
8 1.70848885848761
9 2.54706733125846
10 2.68280914008794
11 3.03836006023276
12 2.97587855246912
13 2.33742548847382
14 1.6707853644491
15 0.890169824566778
16 0.470820173063712
17 -0.249657367634093
18 -0.949598688946624
19 -1.28977649422348
20 -1.74415558918916
21 -2.0989513156621
22 -2.57805246226989
23 -3.28089910172165
24 -4.0633131140578
25 -4.76322410476811
26 -5.28518670439999
27 -5.82559461636148
28 -6.37178329402157
29 -7.04366315558309
};
\addplot [semithick, color1, opacity=0.3]
table {%
0 2.5580886040598
1 2.05050299682174
2 0.847305849562487
3 0.275190515052861
4 0.366950746757768
5 0.284062018291825
6 0.924666698642934
7 2.02269330602111
8 3.29365111694727
9 4.37403232711213
10 5.07814402481453
11 5.09571793518911
12 4.68406353714561
13 4.17485982245585
14 3.30300432263486
15 2.66784308697929
16 1.82389689920837
17 1.16314746224602
18 0.609422091887255
19 -0.295952359600266
20 -0.968389308322893
21 -1.50177547770001
22 -2.18035839050538
23 -2.86868794945984
24 -3.58367840060782
25 -4.3391752620356
26 -5.14406863963293
27 -5.81308439349446
28 -6.66324079639169
29 -7.47345429664766
};
\addplot [semithick, color1, opacity=0.3]
table {%
0 2.18580511457684
1 1.33590704498062
2 0.0457505938324569
3 -0.624997860664665
4 -0.785059151072595
5 -1.09156770646567
6 -1.25096876405481
7 -0.499318713627915
8 0.298399885267777
9 0.935245817784919
10 1.0486318229443
11 1.48323634865919
12 1.14068201264867
13 1.07021570771394
14 0.757704382184178
15 0.169733361260159
16 -0.325675562695025
17 -0.60460362127097
18 -1.10765978500892
19 -1.49797524033272
20 -1.77891282510287
21 -2.06891205860326
22 -2.54857680700819
23 -2.82639740102089
24 -3.30681326763118
25 -3.89024932902147
26 -4.36782182689735
27 -4.80204794876986
28 -5.30525321589301
29 -5.957711816799
};
\addplot [semithick, color1, opacity=0.3]
table {%
0 2.47304667391637
1 1.68062254004544
2 0.649524694665191
3 -0.202394465895555
4 0.0918701584306074
5 0.0832258855982424
6 0.223745130063396
7 0.726596057600378
8 1.76096927582822
9 2.84158747712249
10 3.55581721606261
11 4.22164584145776
12 3.63451347056828
13 2.96503423549254
14 1.9336174990139
15 1.06817454073297
16 0.102471154523364
17 -0.806743666234567
18 -1.74993088143967
19 -2.48582410965282
20 -3.18524392537601
21 -3.85724088240602
22 -4.72102813598256
23 -5.30417671784578
24 -6.15588790717525
25 -7.29246338509665
26 -8.17122887843664
27 -8.85881345499617
28 -9.64784536790648
29 -10.5220338861082
};
\addplot [semithick, color1, opacity=0.3]
table {%
0 2.71180745484452
1 2.13327849584911
2 0.962815638489248
3 0.102670427157252
4 0.390486774376294
5 0.513050201105806
6 1.37843963333861
7 2.39271652110924
8 3.39582954529271
9 4.23939991215617
10 4.56199907826469
11 4.51313852953463
12 4.29548046032312
13 3.97912552209978
14 3.32635510241958
15 2.74421997750359
16 1.873862121793
17 1.28223475335211
18 0.860889035211358
19 0.0453110621840835
20 -0.540301251623044
21 -1.30155181756695
22 -2.29992285553088
23 -3.04680102311592
24 -4.03201658415171
25 -5.069718277824
26 -6.08729718353822
27 -7.13830699056134
28 -8.10892743023669
29 -9.22717693360346
};
\addplot [semithick, color1, opacity=0.3]
table {%
0 2.6318276695961
1 1.96288238028836
2 0.915866241023757
3 0.406831109611323
4 0.801981944913969
5 1.40876703911327
6 2.43842265875765
7 3.70162939102626
8 4.71182030846206
9 5.49079531856058
10 6.27292169445496
11 6.86693778150386
12 6.69076733859369
13 6.41585531730658
14 6.07746476885682
15 5.77697672473427
16 5.76796859281252
17 5.91729156106864
18 5.83268919829703
19 6.04737954810041
20 6.28557449647825
21 6.42150842119987
22 6.74948269018679
23 7.05552824752717
24 7.10572437073244
25 7.47260506530455
26 7.93734909945906
27 8.06229963023739
28 8.4525692132425
29 8.74841219932729
};
\addplot [semithick, color1, opacity=0.3]
table {%
0 2.67953268899794
1 2.10772921570662
2 1.17859165476992
3 0.692929299844977
4 1.35335448850732
5 1.62381417829932
6 1.96130322774569
7 3.32093791030863
8 4.36826111689517
9 5.22277891702188
10 5.44027830948928
11 6.03542213980876
12 5.80857946988982
13 5.08827144202809
14 4.46939932312814
15 3.87166518090771
16 3.07902652792793
17 2.69790672034229
18 2.29441207586672
19 1.65411525755188
20 1.33248486307257
21 0.708084973493079
22 0.112857735630183
23 -0.287795506081338
24 -1.18871614006775
25 -1.82530989620391
26 -2.50472068424581
27 -3.21203104063378
28 -3.85729963044603
29 -4.55744174555877
};
\end{groupplot}

\begin{groupplot}[group style={group size=1 by 3}]
\nextgroupplot[
xshift=-8,
xmin=-1.45, xmax=30.45,
ymin=2.7, ymax=6.7,
width=\figurewidth,
height=\figureheight,
xtick={},
xticklabels={},
yticklabels={},
tick align=outside,
tick pos=left,
x grid style={white!69.019607843137251!black},
y grid style={white!69.019607843137251!black}
]
\addplot [line width=0.06pt, color0, mark=*, mark size=2, mark options={solid,draw=black}]
table {%
0 3.31996634253658
1 3.45443899460193
2 3.38784218387077
3 3.01931286439371
4 2.82906626173755
5 3.09427938765557
6 3.60416870184349
7 4.24596487007442
8 4.84338888587772
9 5.27994908427636
10 5.61004074039071
11 5.90268352537916
12 6.05852129333431
13 6.16858387553312
14 6.19509636026208
15 6.21485180933973
16 6.20378189365436
17 6.1468591562609
18 6.14787992255152
19 6.14579317317396
20 6.15283082950704
21 6.15412613868876
22 6.14366281427887
23 6.16587792193215
24 6.18223254289368
25 6.18638821201769
26 6.14794417270148
27 6.14179954980725
28 6.15812095860932
29 6.16746194810668
};
\end{groupplot}

\begin{groupplot}[group style={group size=1 by 3}]
\nextgroupplot[
xshift=-8,
xmin=-1.45, xmax=30.45,
ymin=-0.85, ymax=5.85,
width=\figurewidth,
height=\figureheight,
xtick={},
xticklabels={},
yticklabels={},
axis y line=right,
tick align=outside,
xtick pos=left,
ytick pos=right,
x grid style={white!69.019607843137251!black},
y grid style={white!69.019607843137251!black}
]
\addplot [line width=0.06pt, color1, mark=*, mark size=2, mark options={solid,draw=black}]
table {%
0 2.65103446372252
1 1.87298481713709
2 1.03310235020523
3 -0.0349224785257646
4 -0.681923979276541
5 -0.614035490335335
6 -0.208100847346677
7 0.33428430837777
8 0.710486243049944
9 0.726233644866842
10 0.520411660737353
11 0.347599665643602
12 0.244300607278545
13 0.195112904269273
14 0.20629800498181
15 0.161911176310666
16 0.161283251423433
17 0.247899352697984
18 0.208651205023874
19 0.171253015388636
20 0.20029198108343
21 0.172890109571832
22 0.187770311286831
23 0.213147053788955
24 0.185796243819713
25 0.165625930691843
26 0.187584184388062
27 0.20252014981221
28 0.179459395114634
29 0.2013127196102
};
\end{groupplot}
