# Supplementary material for: Identification of Gaussian Process State Space Models
Source: arXiv:1705.10888 source file (2017-11-07)
Supplement: Supplementary file 3 [file tikz_samples_ep-8-all.tex]

\definecolor{color0}{rgb}{0.12156862745098,0.466666666666667,0.705882352941177}
\definecolor{color1}{rgb}{1,0.498039215686275,0.0549019607843137}

\begin{groupplot}[group style={group size=1 by 3}]
\nextgroupplot[
xshift=-8,
title={8 episodes},
title style={font=\large},
xmin=-1.45, xmax=30.45,
ymin=2.7, ymax=6.7,
width=\figurewidth,
height=\figureheight,
xtick={},
xticklabels={},
yticklabels={},
tick align=outside,
tick pos=left,
x grid style={white!69.019607843137251!black},
y grid style={white!69.019607843137251!black}
]
\addplot [semithick, color0, opacity=0.3]
table {%
0 3.48337875869527
1 3.6442202037301
2 3.66282466808451
3 3.36453350774775
4 3.27965046788557
5 3.29208727891878
6 3.39261136185822
7 3.45003434238356
8 3.28031762306548
9 2.98757875182044
10 2.78244171044778
11 2.72029312396403
12 2.48995444583512
13 2.26150669313712
14 2.05177589427387
15 1.84316686578503
16 1.64678010962233
17 1.48731584272048
18 1.26190536714608
19 1.10980469739296
20 0.796799009314428
21 0.679425175258739
22 0.373051054486364
23 0.0659012195365154
24 -0.182576403015553
25 -0.564756018533565
26 -0.953884405591626
27 -1.2728656887166
28 -1.71057071845999
29 -2.14930639957504
};
\addplot [semithick, color0, opacity=0.3]
table {%
0 3.75692694683593
1 4.01014900262247
2 3.84176781894086
3 3.47793920274067
4 3.38911663383903
5 3.63948850617803
6 3.88004880307313
7 3.98895927965018
8 3.87870065992497
9 3.93332641368873
10 3.79027531766603
11 3.83766111162598
12 3.64323390690747
13 3.43222694513809
14 3.20386024669403
15 2.97112072254271
16 2.73532236190239
17 2.79499737448877
18 3.08226953384808
19 3.50520445560815
20 3.83785745327285
21 4.06772072217622
22 4.12065818974769
23 3.99816253559129
24 3.74832459086682
25 3.33470852038491
26 3.10118519038182
27 3.10661933782059
28 3.19068114809326
29 3.47441749704563
};
\addplot [semithick, color0, opacity=0.3]
table {%
0 3.65234732581682
1 3.90010842653655
2 3.63938621913213
3 3.36216327308807
4 3.32203809417704
5 3.63120797879368
6 3.9928402058386
7 4.07817832344486
8 4.23180001394492
9 4.40839427054663
10 4.51243257420724
11 4.56874205781971
12 4.41662005422091
13 4.38088843028637
14 4.38447991144576
15 4.41665054810174
16 4.30117435453017
17 4.18020512972514
18 4.14805723336751
19 3.95851209545402
20 3.8557265033704
21 3.98884736350419
22 4.12402241911154
23 4.33147122547376
24 4.50298236677333
25 4.60929015112806
26 4.5918796656371
27 4.45418341405489
28 4.2941886562424
29 4.16389658239248
};
\addplot [semithick, color0, opacity=0.3]
table {%
0 3.75122655419372
1 4.07901111583593
2 3.8984151782181
3 3.61417579327541
4 3.48566880818386
5 3.6979929692895
6 3.98859862505109
7 4.00313004113371
8 3.92224789987416
9 4.14703322285152
10 4.4331853079169
11 4.91805343191512
12 5.4003906763876
13 5.81160735787195
14 5.95016323116149
15 6.08444721693215
16 5.79036059685789
17 5.50478027071253
18 5.19288623253458
19 5.07790749538615
20 4.93931117889542
21 4.98050369649413
22 5.18343388000498
23 5.37599817667426
24 5.61256760108844
25 5.84456361250139
26 5.89711292267137
27 5.97847317601459
28 5.92382737928073
29 5.8989496494955
};
\addplot [semithick, color0, opacity=0.3]
table {%
0 3.6568350896717
1 4.02176498329454
2 4.05344731636131
3 3.74774990808631
4 3.67932077661175
5 3.75331385075798
6 3.74208352467637
7 3.60409617440468
8 3.53846299141638
9 3.47710327277611
10 3.23195537667875
11 3.17478822566972
12 2.91958263313008
13 2.45672519236248
14 1.90549630231465
15 1.25486578675158
16 0.807087184272254
17 0.291396411928766
18 0.00064833090104699
19 -0.363798879794606
20 -0.570911397091843
21 -0.912194161316233
22 -1.40494077120224
23 -1.92064285974698
24 -2.47878285434533
25 -2.98364535849569
26 -3.4509188483338
27 -3.78892201317439
28 -4.16632372416114
29 -4.57639451005674
};
\addplot [semithick, color0, opacity=0.3]
table {%
0 3.87098666412201
1 4.12093277573055
2 3.98626372845992
3 3.82698242426428
4 3.76036070108147
5 3.82944860022407
6 3.76362125608429
7 3.68189982114874
8 3.47336439679899
9 3.85813465387593
10 4.26266344937843
11 4.68812783526384
12 4.98562372080937
13 5.12711303054221
14 5.23147767073895
15 5.02608680465105
16 4.74697212501896
17 4.4848599318816
18 4.30556152782077
19 4.08820107866623
20 3.87440167315797
21 3.94087801353455
22 4.10863244160597
23 4.2820411330909
24 4.51494352332015
25 4.69024004908491
26 4.71061148432857
27 4.77384674269846
28 4.81829433956539
29 4.91505539191804
};
\addplot [semithick, color0, opacity=0.3]
table {%
0 3.53945268349674
1 3.7370250177998
2 3.68028427583068
3 3.64278633528485
4 3.69759559145772
5 3.84883842628306
6 3.98228073317847
7 4.00170976660768
8 4.11107631725844
9 4.30248595941989
10 4.30968685920947
11 4.25912925325406
12 4.13381932570561
13 3.840099870979
14 3.62609213468741
15 3.41363410695543
16 3.13743502739556
17 3.06650851868855
18 3.23579179701332
19 3.49623781782729
20 3.8919297974781
21 4.24568418796184
22 4.58389358413321
23 4.73877594357643
24 4.72321095988689
25 4.54276335747558
26 4.319444191326
27 4.19624900353447
28 4.12218697444437
29 4.19400406398713
};
\addplot [semithick, color0, opacity=0.3]
table {%
0 3.73574178546096
1 4.01898640462085
2 3.97435821108532
3 3.78860290919008
4 3.72443461978893
5 3.99558092297967
6 4.14504007228924
7 4.25032624223739
8 4.32940692966766
9 4.5331160994636
10 4.63553918079801
11 4.72117706494963
12 4.65596791231052
13 4.34970658445617
14 4.43074221078944
15 4.46937307417792
16 4.4302042920591
17 4.39232182210118
18 4.38447372454579
19 4.38271915111191
20 4.25407018154569
21 4.25723872422524
22 4.40287483881216
23 4.54507908619838
24 4.55557864473132
25 4.58373300239576
26 4.52423415306044
27 4.45531896393169
28 4.48153041254366
29 4.57918336539489
};
\addplot [semithick, color0, opacity=0.3]
table {%
0 3.75485920290594
1 3.96842605176422
2 3.80900874237053
3 3.67144964057277
4 3.53701625967359
5 3.70182056516957
6 3.74456148580934
7 3.88169332084518
8 4.08262721583412
9 4.29454231544214
10 4.44244093324172
11 4.61186135261001
12 4.4676483576001
13 4.26831067437921
14 4.06192383422567
15 3.98394533792294
16 3.85617648780099
17 3.95910019502746
18 4.21436553140894
19 4.45294936824948
20 4.68299498329539
21 4.91428368556922
22 5.12172771363984
23 5.12133269429512
24 5.22824201419339
25 5.33394286079186
26 5.30985192593281
27 5.27382060165261
28 5.27268445194817
29 5.25289193551714
};
\addplot [semithick, color0, opacity=0.3]
table {%
0 3.69581243955628
1 3.91887573365133
2 3.87355098313053
3 3.53003109168975
4 3.48337107751317
5 3.73233264825417
6 3.91737820902166
7 3.75168074706782
8 3.56900913848411
9 3.42263408566148
10 3.22737774852689
11 2.82983146349931
12 2.39860326926466
13 1.93102289003277
14 1.54121694104587
15 1.17581164637895
16 0.997737779186016
17 0.644961519609529
18 0.380081086889344
19 -0.052271940784701
20 -0.572752593366785
21 -1.09203909161029
22 -1.60500772762445
23 -2.15046281788578
24 -2.70473998409462
25 -3.30946770521974
26 -3.84737504233836
27 -4.35473942952219
28 -4.90375584205518
29 -5.36077982413389
};
\addplot [semithick, color0, opacity=0.3]
table {%
0 3.7856298254202
1 4.09630485351153
2 4.08807681540183
3 3.88651958075562
4 3.87183050240927
5 4.02412001602768
6 4.05030855418972
7 3.97514465244214
8 3.84120715810627
9 3.78155396382583
10 3.59643393078013
11 3.53863554949776
12 3.04598396354397
13 2.52456652994421
14 1.98818312964271
15 1.54888723283305
16 1.25733960870063
17 1.09578124516476
18 1.04394400759814
19 1.26512378284637
20 1.3880493830703
21 1.50354769614053
22 1.53277698941767
23 1.28199883492338
24 1.03871081771662
25 0.532317805528981
26 0.0781959945317521
27 -0.309353433490054
28 -0.894413262014664
29 -1.57284514716435
};
\addplot [semithick, color0, opacity=0.3]
table {%
0 3.64573686481737
1 3.78479644012612
2 3.75901502677705
3 3.66378648182119
4 3.67290209807681
5 4.03135821590982
6 4.15136894290023
7 4.01247280852929
8 3.92282489750376
9 3.80499433663094
10 3.88970247250222
11 3.91506837853817
12 3.87490231586382
13 3.85250290953584
14 3.860039844322
15 3.88171267365335
16 3.75335582017392
17 3.58179325539474
18 3.28797457128038
19 2.9332741259104
20 2.61218971624792
21 2.54116643642831
22 2.53828301484527
23 2.53805660596948
24 2.67163961361724
25 2.74805339078508
26 2.82904708945047
27 2.81904394945592
28 2.84575252593818
29 2.83783689860793
};
\addplot [semithick, color0, opacity=0.3]
table {%
0 3.71763152540294
1 3.94605377228024
2 3.57434577967726
3 3.08827707115009
4 2.90157722278035
5 3.05261601262763
6 3.21223813928705
7 3.45599048309542
8 3.44898015216311
9 3.5824886263218
10 3.81327465312553
11 3.99714693215204
12 3.84115332463437
13 3.77098343302155
14 3.58834515695817
15 3.47451379665512
16 3.17809394347855
17 3.00091365021702
18 2.8963732222488
19 2.92421569406842
20 2.98605587128072
21 3.1748592334647
22 3.35298842338556
23 3.51828345761705
24 3.51492586433345
25 3.52824549606665
26 3.51787899330005
27 3.42194571217321
28 3.41270635041167
29 3.3535310767473
};
\addplot [semithick, color0, opacity=0.3]
table {%
0 3.92980368462784
1 4.15241060259077
2 3.90172987815915
3 3.66475666036754
4 3.30507022544961
5 3.357641997975
6 3.55206162297724
7 3.9116867954236
8 4.10419848614916
9 4.35367103534581
10 4.6227383789132
11 4.62185851001647
12 4.43356851381904
13 4.25250268985707
14 3.93726871410397
15 3.73991025176629
16 3.61441611335777
17 3.61813900023431
18 3.68221689399896
19 4.16111406013854
20 4.45168793674757
21 4.85080669672653
22 5.2668314934224
23 5.5150248465053
24 5.73160684788407
25 5.85624776741652
26 5.88191360876757
27 5.84502060973749
28 5.9267994373716
29 5.8496709670095
};
\addplot [semithick, color0, opacity=0.3]
table {%
0 3.87541415708238
1 4.08993418870803
2 3.89007595517407
3 3.6310241125162
4 3.47161634574683
5 3.47562892044868
6 3.56878422847304
7 3.56202867533099
8 3.51883732818689
9 3.61514470518779
10 3.9013164792277
11 4.13197184761291
12 4.39868122377741
13 4.48162402988892
14 4.55060530801949
15 4.653854028617
16 4.78185489540605
17 4.95556724952147
18 5.03780537232518
19 4.9234087081531
20 4.85457549910474
21 4.95426343560363
22 4.94507110878404
23 5.039250050742
24 5.3380246735513
25 5.62880775370637
26 5.71056846373902
27 5.72706488201095
28 5.57354318609019
29 5.4780129749678
};
\addplot [semithick, color0, opacity=0.3]
table {%
0 3.64242913543583
1 3.96247246668598
2 3.97072102534323
3 3.95465564375668
4 3.87088855458676
5 4.05911801007885
6 4.37459654142961
7 4.49434582700594
8 4.28262598082436
9 4.28054974233086
10 4.35451886161533
11 4.45626355116605
12 4.47763722476805
13 4.55406385398167
14 4.71153092192055
15 5.02889564673771
16 5.14992632579977
17 5.06680425515105
18 4.98444755585941
19 4.86475602048422
20 4.84508077642069
21 4.90957164005385
22 4.93391910464057
23 5.17727019515626
24 5.39718387152821
25 5.67522479801721
26 5.78519524786402
27 5.87470225566531
28 5.94729254902164
29 5.94398573843628
};
\addplot [semithick, color0, opacity=0.3]
table {%
0 3.7456656750272
1 3.98084573429858
2 3.9296144290903
3 3.73484504914595
4 3.61867234557538
5 3.84451748054673
6 4.0348780224517
7 4.2962093783034
8 4.38990889151089
9 4.44354752581499
10 4.51218109274764
11 4.47223181956849
12 4.30392685969749
13 4.41064217800854
14 4.57823613268433
15 4.87551822424888
16 5.09090140723769
17 5.26958621080005
18 5.44557232971366
19 5.57430796679935
20 5.63337246923994
21 5.58948045633056
22 5.64778943384696
23 5.77819391547392
24 5.89577373898171
25 6.00972748227465
26 6.2193326050542
27 6.47318808559541
28 6.59146714210536
29 6.72948702875354
};
\addplot [semithick, color0, opacity=0.3]
table {%
0 3.87288789603665
1 4.17483681681896
2 4.17654543231314
3 3.89192263230608
4 3.68899188935305
5 3.83030574414674
6 3.95993059621402
7 4.16920489951448
8 4.35464511489283
9 4.56620365645315
10 4.60299826153757
11 4.41666146905337
12 4.10182197078316
13 3.58485562097327
14 2.9564504615239
15 2.57991697073926
16 2.47810896146473
17 2.49475192443373
18 2.77479784294432
19 3.3011060565353
20 3.65054397658144
21 4.12763154281841
22 4.39023998964417
23 4.23750570425577
24 3.9932291138581
25 3.54114971315715
26 3.23682900952312
27 3.08468640088209
28 3.11253884174229
29 3.3776434988986
};
\addplot [semithick, color0, opacity=0.3]
table {%
0 3.86026056634126
1 4.28954618265937
2 4.31331348028386
3 4.34915544162042
4 4.25169277820764
5 4.31180610780142
6 4.27292372548523
7 4.16590675858998
8 4.06560010306182
9 4.10801917742977
10 4.07055872339201
11 3.96181968366082
12 3.64938985951848
13 3.51517454070201
14 3.39227779562857
15 3.48092321318838
16 3.53291887738918
17 3.6609868213714
18 3.85217669065652
19 3.9784678862473
20 3.99998827425934
21 4.09290629574085
22 4.2508733701415
23 4.24897287735535
24 4.50461026137931
25 4.63366439529667
26 4.80312787783364
27 4.81577093102074
28 4.9506379945922
29 5.18886836218157
};
\addplot [semithick, color0, opacity=0.3]
table {%
0 3.69712382969966
1 3.92212007735063
2 3.82703785211794
3 3.71092597942983
4 3.74075887807424
5 3.80974547115642
6 3.86134445003896
7 3.71046819196614
8 3.36498374618602
9 3.10754142822998
10 2.89982910841615
11 2.63175301397082
12 2.12231827583077
13 1.51655739657703
14 1.05028941892878
15 0.432784400725952
16 -0.032415520205074
17 -0.516637340562635
18 -1.08757342130684
19 -1.69080507993
20 -2.27253035985337
21 -2.76849265246961
22 -3.33529575350975
23 -3.73400561520718
24 -4.21803253716014
25 -4.73043950328871
26 -5.28384382850145
27 -5.76341763501967
28 -6.23442454821156
29 -6.69810738871337
};
\end{groupplot}

\begin{groupplot}[group style={group size=1 by 3}]
\nextgroupplot[
xshift=-8,
xmin=-1.45, xmax=30.45,
ymin=-0.85, ymax=5.85,
width=\figurewidth,
height=\figureheight,
xtick={},
xticklabels={},
yticklabels={},
axis y line=right,
tick align=outside,
xtick pos=left,
ytick pos=right,
x grid style={white!69.019607843137251!black},
y grid style={white!69.019607843137251!black}
]
\addplot [semithick, color1, opacity=0.3]
table {%
0 1.99461017672552
1 0.827397330337661
2 -0.377487921631158
3 -1.64492547155563
4 -2.67206975415198
5 -3.69021788830489
6 -3.74518413527199
7 -2.99427166820469
8 -2.06917161658307
9 -1.39218209477295
10 -1.21058707882414
11 -0.999428943155051
12 -1.02640819823377
13 -1.22678118019291
14 -1.43760087933121
15 -1.94543140707707
16 -2.50283519333045
17 -3.43898295261109
18 -4.58058081199334
19 -5.80160665527764
20 -7.2526037237346
21 -8.59529989589816
22 -9.8473458968948
23 -10.7755097979289
24 -11.7731676881498
25 -12.5747008248684
26 -13.0842068585951
27 -13.6985481759729
28 -14.1931084595232
29 -14.6971176429522
};
\addplot [semithick, color1, opacity=0.3]
table {%
0 2.39885257478199
1 1.55443614941206
2 0.363775882548737
3 -0.715888628494877
4 -1.41098340476658
5 -1.79131499472773
6 -1.75987184283016
7 -1.07424956211091
8 0.0294015827155558
9 0.760981984249575
10 1.13992533208294
11 1.70952542120269
12 1.96812308357942
13 2.10346420866903
14 2.10002176401301
15 2.40504847763257
16 2.48853501838962
17 2.72327801194155
18 2.41254642598856
19 2.03966301170832
20 1.73135152742586
21 1.53896462944886
22 1.58965481522817
23 1.88414214001336
24 2.03060655753461
25 2.32300074684652
26 2.66529131036937
27 2.78458313951143
28 2.86213343524897
29 2.89731874313489
};
\addplot [semithick, color1, opacity=0.3]
table {%
0 2.45453667866042
1 1.56836218173971
2 0.437027028580443
3 -0.250968720457816
4 -0.850396281877552
5 -0.887731136219344
6 -0.695649682254547
7 0.18295530252189
8 1.49829773060017
9 2.01038624121872
10 2.64452353647915
11 3.32965000511349
12 3.47231365988185
13 3.52977177435953
14 3.22968726230891
15 3.30866852167292
16 3.27779550663195
17 3.34369546361843
18 3.3626177961707
19 3.54406863515322
20 3.61243556870935
21 3.411023115105
22 3.43992837487628
23 3.30100753664147
24 3.24215446229016
25 3.23071933553916
26 3.25986540329249
27 3.39333146121557
28 3.43120747256236
29 3.4842488375827
};
\addplot [semithick, color1, opacity=0.3]
table {%
0 2.69278778085465
1 1.93847872297612
2 1.08393553059563
3 0.370487022229572
4 -0.000395202589444921
5 0.199780089976102
6 0.80598326953789
7 2.0642637708215
8 3.48396042277964
9 4.01199124517597
10 4.38612333467757
11 4.49218518940418
12 4.27722473596879
13 4.21668129641129
14 4.12173800000473
15 3.99160592307866
16 4.33232089623921
17 4.56597259430976
18 4.7832323668745
19 4.9495786645893
20 5.05304518773267
21 4.80779822101048
22 4.63961280789511
23 4.5838666461479
24 4.50931229560942
25 4.573450127647
26 4.7615920736987
27 4.85399115580068
28 5.03508577085903
29 5.3866927420163
};
\addplot [semithick, color1, opacity=0.3]
table {%
0 2.35216456807257
1 1.24327038488901
2 -0.0163412927321858
3 -1.25186424740748
4 -2.18334113346784
5 -2.81567564037371
6 -3.01421923451723
7 -2.80932471740986
8 -1.89986718714576
9 -1.51502945525684
10 -1.61947417153253
11 -1.77520147002146
12 -2.3950257260827
13 -3.00909083582242
14 -3.74049262718714
15 -4.67108780532389
16 -5.74323480664615
17 -7.29677061422106
18 -8.58509214482359
19 -9.8117957230651
20 -10.9919059736211
21 -12.125924946692
22 -13.3323290490169
23 -14.3469684935679
24 -15.2632391852358
25 -16.2806101153986
26 -16.9399298358848
27 -17.4050907132992
28 -17.8163687153338
29 -18.4991648773121
};
\addplot [semithick, color1, opacity=0.3]
table {%
0 2.30959573012918
1 1.71001221143436
2 1.07792430693352
3 0.630574984997118
4 0.238518206383945
5 0.55458898592436
6 1.28765230673705
7 2.43499858847068
8 3.8359970248021
9 4.38673216308278
10 4.55980538581475
11 4.39370559018588
12 4.06441473371834
13 3.76393128808139
14 3.44103223303614
15 3.41296758731246
16 3.6918680470943
17 3.74401876843425
18 3.94912980136757
19 4.12312268376747
20 4.21150206604718
21 4.33613158699382
22 4.57374589311995
23 4.64175408549407
24 4.66109880833776
25 4.69239736275476
26 4.80210300178135
27 4.84328517702675
28 4.88064707792347
29 5.01074844574788
};
\addplot [semithick, color1, opacity=0.3]
table {%
0 2.43537759705551
1 1.42770184040541
2 0.531578421509849
3 -0.258310275883611
4 -1.02814237389804
5 -1.1794671908212
6 -0.863403138503735
7 -0.241837028697741
8 0.506012988701126
9 1.13750094304367
10 1.50177798788923
11 1.92651926148077
12 2.37060297888604
13 2.47140928565647
14 2.53518533232527
15 2.79748562464407
16 2.9904419924704
17 3.21683854092459
18 3.28987769294083
19 3.08117457845938
20 2.9687271346252
21 2.73474373412524
22 2.60560417673512
23 2.68175781865171
24 2.78344654034236
25 2.93578554935012
26 3.29794851398456
27 3.61367019420044
28 4.00912280959897
29 4.30070449146154
};
\addplot [semithick, color1, opacity=0.3]
table {%
0 2.52021851563423
1 1.74057020148982
2 0.70178589580803
3 -0.216971289859018
4 -0.688047392577126
5 -0.757927881514766
6 -0.446378266058659
7 0.624642292694491
8 1.8676978421172
9 2.71377397681399
10 3.40427192225047
11 3.94256248929903
12 4.13363532725283
13 4.06122607914693
14 3.87980434338915
15 3.56447828113606
16 3.56562801946567
17 3.7254204997124
18 3.72541252003617
19 3.79984256048527
20 4.03452139612418
21 3.98312822768021
22 4.1269054438837
23 4.23883179550966
24 4.11575846823425
25 4.20356512308793
26 4.26187888183372
27 4.44056774113485
28 4.4640294542653
29 4.4737999475353
};
\addplot [semithick, color1, opacity=0.3]
table {%
0 2.2622638127073
1 1.31457929488215
2 0.149301934569104
3 -0.631879977314568
4 -1.06243692984532
5 -0.963550801353517
6 -0.761578516401904
7 -0.0652961704663078
8 0.903469093868605
9 1.59417778421812
10 2.34375470677474
11 2.88262834619849
12 3.19917768620117
13 3.41043355739356
14 3.56354029160057
15 3.57409217186134
16 3.71271186645883
17 3.91317294518803
18 3.75479286026351
19 3.76597359900927
20 3.84959483790308
21 3.98566172861346
22 4.20409209925658
23 4.4116043987448
24 4.47473863800988
25 4.58485086627765
26 4.8869841909284
27 5.02316143460424
28 5.07075439318583
29 5.20799963162311
};
\addplot [semithick, color1, opacity=0.3]
table {%
0 2.0096791884375
1 0.991040172776348
2 -0.349900104366517
3 -1.69591702568425
4 -2.6480725993295
5 -3.15119800940822
6 -3.11063539331121
7 -2.3491935521829
8 -1.47333738704934
9 -1.08285199741858
10 -1.02890678144074
11 -0.978053782451926
12 -1.32633995053428
13 -1.81315707372143
14 -2.50290578209164
15 -3.73739643229942
16 -4.86934974312708
17 -6.31942612840846
18 -7.8210633487278
19 -9.66724467069437
20 -11.1738707487261
21 -12.4662530491203
22 -13.6519861296607
23 -14.7908742181902
24 -15.6714679033192
25 -16.4654488967341
26 -17.0486489423882
27 -17.951383902638
28 -18.5518655748988
29 -18.873797965001
};
\addplot [semithick, color1, opacity=0.3]
table {%
0 2.36765378651552
1 1.38499440579082
2 0.352797392947577
3 -0.348362883308786
4 -1.08861964138042
5 -1.60678911772122
6 -2.08234970138046
7 -1.92193626485633
8 -0.961391333835175
9 -0.578765012153761
10 -0.329685360363662
11 -0.0952719997615414
12 -0.404077637513396
13 -0.822431956061342
14 -1.1548590729542
15 -1.55913240732626
16 -1.87474737016176
17 -2.04942789997101
18 -2.42167226596014
19 -2.83377062773073
20 -3.44409749497884
21 -4.0801649931814
22 -4.76395739210256
23 -5.89806115295164
24 -6.84710702604742
25 -7.95998801140924
26 -9.08726140834647
27 -10.1368964012825
28 -11.1354449978007
29 -12.1443297476642
};
\addplot [semithick, color1, opacity=0.3]
table {%
0 2.19343832813298
1 1.41863170980538
2 0.661251604152236
3 -0.132150962436018
4 -0.864338689445006
5 -1.21238449552417
6 -1.24577358153776
7 -0.583723388590824
8 0.55931500134024
9 1.16795499352602
10 1.8198345539299
11 2.26705237508012
12 2.29866624137685
13 2.14546857633499
14 1.89232471670018
15 1.67957613114191
16 1.5200406815462
17 1.51876825311286
18 1.44519131607588
19 1.5304428144022
20 1.50580497370789
21 1.49813635383157
22 1.52930810094324
23 1.34711794947988
24 1.2858503073271
25 1.11465652030522
26 0.819498176471054
27 0.714513842417864
28 0.498256467901353
29 0.166702256362214
};
\addplot [semithick, color1, opacity=0.3]
table {%
0 2.42506003689749
1 1.43668541112496
2 0.244011318021105
3 -0.691783203000709
4 -1.21728588065206
5 -1.50031501692393
6 -1.39058077128278
7 -0.789821543144868
8 0.0584214923778799
9 0.776473799667331
10 1.25753318674992
11 1.65176227783974
12 1.70195584692446
13 1.8586433336953
14 1.92322666054159
15 1.84486559602889
16 1.71571280180357
17 1.6934161056575
18 1.5768235822147
19 1.79725469992804
20 1.8225383859363
21 1.82149847089649
22 1.79780594102779
23 1.83747040264958
24 1.56629636391772
25 1.3281376145392
26 1.28567937271598
27 1.35485683917309
28 1.41161687823879
29 1.42005945078185
};
\addplot [semithick, color1, opacity=0.3]
table {%
0 2.30798502231453
1 1.30414353422589
2 0.275243571559624
3 -0.557516364962629
4 -1.01907860176867
5 -1.25320946117963
6 -1.0852305206993
7 -0.490600230746743
8 0.62923826594894
9 1.2079251631749
10 1.87720002025102
11 2.28429159778494
12 2.77743825153589
13 3.10638991955788
14 3.55088136076224
15 3.77043008321806
16 4.13469151530509
17 4.45436182057677
18 4.59188842445298
19 4.77968126547275
20 5.09485810486102
21 5.36199972523518
22 5.60259516830553
23 5.88816389569383
24 6.03643253986177
25 6.30199957581043
26 6.67312346677868
27 7.02153230872913
28 7.39415096620553
29 7.76134983280909
};
\addplot [semithick, color1, opacity=0.3]
table {%
0 2.2555166824542
1 1.4348837961966
2 0.349149177428572
3 -0.528626257165866
4 -1.0981389727185
5 -1.33261845365992
6 -1.10266382602354
7 -0.279496660733933
8 0.865199620078856
9 1.68341059486656
10 2.31960372513849
11 2.82674821635305
12 3.24974316588945
13 3.3362305517646
14 3.29799938364185
15 3.28907604885197
16 3.33535274324892
17 3.49007050826604
18 3.74417707055337
19 3.83849310220018
20 3.98814655522294
21 4.07926757252283
22 4.02780291432875
23 4.17888143103723
24 4.17286931698469
25 4.16455450289857
26 4.24507579101065
27 4.53451530083713
28 4.81511401957661
29 4.64666442088688
};
\addplot [semithick, color1, opacity=0.3]
table {%
0 2.53103163672522
1 1.83836639874313
2 0.805356670882457
3 0.182583293226992
4 -0.470411576220197
5 -0.571610502126893
6 -0.310167164136525
7 0.686287971969948
8 1.63440760004951
9 2.24900961746523
10 2.96742552859612
11 3.57163649790504
12 3.93524804073968
13 3.98882913545796
14 3.94255597960029
15 3.72717690591525
16 3.43862615455369
17 3.5666049709496
18 3.67663364364145
19 4.03406729742686
20 4.37514276378681
21 4.58649666897098
22 4.72927104777996
23 4.56473184178637
24 4.59125224615829
25 4.5273121612386
26 4.66302610674861
27 4.98645046997916
28 5.22790664614146
29 5.53383020046095
};
\addplot [semithick, color1, opacity=0.3]
table {%
0 2.68280213935676
1 1.90706140164081
2 1.01140599143988
3 0.350375216488683
4 -0.21337077865048
5 -0.135720179443565
6 0.265368413986351
7 1.15964252765423
8 2.31877084567818
9 2.96627418066009
10 3.53499161860014
11 4.13680939013969
12 4.73204768491517
13 4.81848540919144
14 4.49890515135081
15 4.42220453541445
16 4.67096089718402
17 4.84817211290194
18 4.9238336531802
19 5.18324308632239
20 5.38521439166348
21 5.5388659531573
22 5.65927350812602
23 5.93501056848117
24 6.17358397513354
25 6.46077202887095
26 6.7999408390064
27 7.00146107459028
28 7.12500284439427
29 7.4487854443086
};
\addplot [semithick, color1, opacity=0.3]
table {%
0 2.21444776014574
1 1.25556248820565
2 0.174639571103585
3 -0.640205734851516
4 -1.17961810884137
5 -1.06674292348844
6 -0.953049654448522
7 -0.349873507361893
8 0.205086394942443
9 0.598082630230902
10 0.969233044158347
11 1.46400749992559
12 1.64555600296063
13 1.92583270680584
14 2.08485696277695
15 2.1397145218112
16 2.3253153020055
17 2.38293768560135
18 2.30295684638456
19 2.23979805435575
20 2.2980117145038
21 2.25201320591605
22 2.2868659239179
23 2.44636192511403
24 2.65001017696619
25 2.72552172224684
26 2.80597952860173
27 2.81577872680342
28 2.79337010199495
29 2.86979817244769
};
\addplot [semithick, color1, opacity=0.3]
table {%
0 2.59578321115962
1 1.72003968291617
2 0.626366092718737
3 -0.151492935504921
4 -0.521001734217201
5 -0.777923050102341
6 -0.523794431534583
7 0.209646787092883
8 0.72562588380293
9 1.1600816713637
10 1.36305400823716
11 1.84755551056985
12 2.23351264192174
13 2.45964565463916
14 2.46732187746045
15 2.50051131676197
16 2.53834745789506
17 2.6759130475762
18 2.67696710219255
19 2.85071609596967
20 3.11257769103067
21 3.21529961429664
22 3.39652038955742
23 3.62964390053373
24 3.83244486499634
25 4.02337913154487
26 4.23143070511489
27 4.5000985954228
28 4.78272447801652
29 4.89276955577757
};
\addplot [semithick, color1, opacity=0.3]
table {%
0 1.90667953803294
1 0.756842711263184
2 -0.418048861923085
3 -1.72528167493683
4 -2.68285990688276
5 -3.57643581221407
6 -4.30971526018273
7 -4.20978809447368
8 -4.05000035344417
9 -4.19600565569071
10 -4.36321779593588
11 -4.7127940364656
12 -5.61082881135376
13 -6.56961664142302
14 -7.61643774724871
15 -8.75620937105619
16 -9.92817796598784
17 -10.8966593935777
18 -11.7790841128455
19 -12.7648066926123
20 -13.4648461113987
21 -14.1321506768745
22 -14.7648404852256
23 -15.2034038572113
24 -15.9628795011629
25 -16.6666734665683
26 -17.1834911352629
27 -17.6404355430797
28 -18.0881163954135
29 -18.6795022254001
};
\end{groupplot}

\begin{groupplot}[group style={group size=1 by 3}]
\nextgroupplot[
xshift=-8,
xmin=-1.45, xmax=30.45,
ymin=2.7, ymax=6.7,
width=\figurewidth,
height=\figureheight,
xtick={},
xticklabels={},
yticklabels={},
tick align=outside,
tick pos=left,
x grid style={white!69.019607843137251!black},
y grid style={white!69.019607843137251!black}
]
\addplot [line width=0.06pt, color0, mark=*, mark size=2, mark options={solid,draw=black}]
table {%
0 3.31996634253658
1 3.45443899460193
2 3.38784218387077
3 3.01931286439371
4 2.82906626173755
5 3.09427938765557
6 3.60416870184349
7 4.24596487007442
8 4.84338888587772
9 5.27994908427636
10 5.61004074039071
11 5.90268352537916
12 6.05852129333431
13 6.16858387553312
14 6.19509636026208
15 6.21485180933973
16 6.20378189365436
17 6.1468591562609
18 6.14787992255152
19 6.14579317317396
20 6.15283082950704
21 6.15412613868876
22 6.14366281427887
23 6.16587792193215
24 6.18223254289368
25 6.18638821201769
26 6.14794417270148
27 6.14179954980725
28 6.15812095860932
29 6.16746194810668
};
\end{groupplot}

\begin{groupplot}[group style={group size=1 by 3}]
\nextgroupplot[
xshift=-8,
xmin=-1.45, xmax=30.45,
ymin=-0.85, ymax=5.85,
width=\figurewidth,
height=\figureheight,
xtick={},
xticklabels={},
yticklabels={},
axis y line=right,
tick align=outside,
xtick pos=left,
ytick pos=right,
x grid style={white!69.019607843137251!black},
y grid style={white!69.019607843137251!black}
]
\addplot [line width=0.06pt, color1, mark=*, mark size=2, mark options={solid,draw=black}]
table {%
0 2.65103446372252
1 1.87298481713709
2 1.03310235020523
3 -0.0349224785257646
4 -0.681923979276541
5 -0.614035490335335
6 -0.208100847346677
7 0.33428430837777
8 0.710486243049944
9 0.726233644866842
10 0.520411660737353
11 0.347599665643602
12 0.244300607278545
13 0.195112904269273
14 0.20629800498181
15 0.161911176310666
16 0.161283251423433
17 0.247899352697984
18 0.208651205023874
19 0.171253015388636
20 0.20029198108343
21 0.172890109571832
22 0.187770311286831
23 0.213147053788955
24 0.185796243819713
25 0.165625930691843
26 0.187584184388062
27 0.20252014981221
28 0.179459395114634
29 0.2013127196102
};
\end{groupplot}
